# Supplementary material for: A Framework for Evaluating Post Hoc Feature-Additive Explainers
Source: arXiv:2106.08376 ancillary file (2022-05-05)
Supplement: Supplementary file 1 [file A_Framework_for_Evaluating_Post_Hoc_Feature-Additive_Explainers_SUPPLEMENTAL.pdf]

# A Framework for Evaluating *Post Hoc* Feature-Additive Explainers

## Supplemental Material

Zachariah Carmichael, Walter J. Scheirer

**Abstract**

The following material provides additional detail for the method and experimental setup, as well as additional experimental results.

## Table of Contents

| | | | |
|---|---|---|---|
| **Appendix A** | **Reproducibility** | **2** |
| **Appendix B** | **Proofs and Derivations** | **8** |
| **Appendix C** | **Additional Results and Figures** | **12** |
| **Appendix D** | **Synthetic Model Generation** | **62** |

## Appendix A Reproducibility

*Model Generation Parameters*

See Algorithm 1 for definitions of parameters. The * in Table A.1 means '1' is implied when $pct_{interact}$ is zero.

| Parameter | Values |
|---|---|
| $d$ | {2, 4, 7, 16, 32, 64, 127, 256, 512, 1024} |
| $n_{dummy}$ | {0, 0.2375$d$, 0.475$d$, 0.7125$d$, 0.95$d$} |
| $pct_{nonlinear}$ | {0, .375, .75, 1.125, 1.5} |
| $pct_{interact}$ | {0, 0.167, 0.333, 0.5} |
| $order_{interact}$ | {1*, 2, 3} |

Table A.1: Model generation parameters

Weights are the probability of being drawn as an operator (normalized against all considered operators in the considered classes). The add operation is only considered when the operator does not break up the interaction effect. The values of $n_{dummy}$ are a function of $d$.

*Explainer Hyperparameters*

In general, the defaults were used and no tuning was performed. We only allowed explainers to explain as many effects as possible as the goal wasn't to produce comprehensible explanations, but rather faithful ones as the only criteria. See the table below for specified parameters of interest. Note that we do not use L1 regularization with `SHAP` as far too many features would be filtered and we do not tune explainer hyperparameters.

*`PDP` Local Explanations*

To generate local explanations using `PDP`, we compute the `PDP` for each feature individually. The `PDPBox` library uses percentiles to sample the domain of each feature. We compute PD for 100 sample points for each feature. Thereafter,

we use linear interpolation between each point, and extrapolation for values outside the range, to give a feature contribution for "unseen" values. The local explanation is thus the interpolated PD of each feature.

*Tiny MNIST*

We evaluate explainers on a down-sampled version of the MNIST dataset as mentioned in the text. Again, all steps taken here are to reduce explainer run-times and improve the comprehensibility of the results. We select a subset of classes to reduce the amount of data and the number of classes to explain. Specifically, we include only the four digits 0, 1, 5, and 8 due to separability between the data of each class. The crop was selected by observing the percentage of non-zero pixels that would be removed for all crop values, i.e., of the top and bottom rows, and the left and right columns. We remove about 1% of all non-zero pixels by using a global crop of 3 pixels from the top, 2 from the bottom, 5 from the left, and 3 from the right. This crop changes each image size from $28 \times 28$ to $23 \times 20$. We then resize each handwritten digit in the dataset to $12 \times 10$ using the `scikit-image` function `resize` with anti-aliasing.

*Experiment Reproducibility*

While all experiments use random seeds, some results may not be completely reproducible due to the behavior of `SymPy` (see the discussion in issue #20522[1]). For instance, the model generation uses the `sympy.calculus.util.continuous_domain` function to determine if generated models have valid input domains. This function randomly iterates through assumptions, and due to bugs, may not converge to the same result. Thus, we provide every `SymPy` model in the `pickle` format, and the generated data, and true contributions, and the explainer contributions in a `NumPy` format. The latter files should not suffer from reproducibility issues, but are provided to guarantee reproducibility. These files are located in a shared Google

[1]`https://github.com/sympy/sympy/issues/20522`

Drive folder: https://drive.google.com/drive/folders/1cBDwi4JIXmAihOv9yfjqrLNsohM-CX5W?usp=sharing.

The source code is also linked in the main paper with the same seeds used in our experiments as the default arguments.

For the neural network, we train each pathway (for each effect) with 3 fully-connected layers [64, 64, 32] with the first two using a ReLU activation and the latter with no activation (identity function). The Adam optimizer is used with a learning rate of 1e-3 and early stopping with a patience of 100 based on the training loss, restoring the best weights at the end of training. The maximum number of epochs is 1,000. For the GAM, a spline term is added with 25 splines for each main effect, and a tensor term with 10 splines per marginal term is used for interaction effects. The link function is logistic for classification and identity for regression.

The convolutional neural network (CNN) uses the same optimization hyper-parameters but a slightly different architecture. The first layer is 2D convolution with a kernel size and stride size of (2, 1), `SAME` padding (i.e., with a stride of one, the filtered output shape is the same as the input shape), and 4 filters. This implies sparsity within the model, thus additive structure. A dense layer then gives the output for each interaction effect from the output of the convolutional layer; due to the kernel and strides sizes, the filter outputs will all comprise the nonlinear ReLU function of 2 features.

For the real-world experiments, data is normalized (z-score normalization) before training. Training uses the full dataset as generalization is not of interest — rather, we only care if explainers can faithfully explain the model's predictions. Feature contributions and data are inverse normalization in all figures for better readability in terms of the underlying features.

*Hardware*

Experiments were run on a cluster running the Univa Grid Engine (UGE) software. Each job was allocated 16 cores of an Intel(R) Xeon(R) CPU E5-2680 v3 @ 2.50GHz and 10 GiB of RAM (soft maximum) per explanation of a model.

Note that by pooling resources, a set of explanation jobs can contend for and pool up to 128 GiB of RAM. The operating system in use was Red Hat Enterprise Linux Server release 7.9 (Maipo). For total time running synthetic experiments, `LIME` took ∼6 hours for all explanations, `SHAP` took ∼18 hours for all explanations, and `MAPLE` exceeded a 2 week budget (although, each run was faster than `SHAP` up until $d > 64$). `SHAPR` exceeded the memory limits for several processes, as well as the time budget of 2 weeks. `PDP` finished all jobs in 6 days.

*Licenses*

The FICO HELOC dataset license is available at `https://community.fico.com/s/explainable-machine-learning-challenge?tabset-3158a=a4c37`. MNIST is under the Creative Commons Attribution-Share Alike 3.0 license. For software, see the corresponding licenses of the cited libraries in the text. Our software is under the MIT License.

| Name | Type | Nonlinear | Weight |
|---|---|---|---|
| $\cosh(\cdot)$ | unary | yes | 0.015 |
| $\cosh(\cdot)$ | unary | yes | 0.015 |
| $\sin(\cdot)$ | unary | yes | 0.015 |
| $\sinh(\cdot)$ | unary | yes | 0.015 |
| $\mathrm{asinh}(\cdot)$ | unary | yes | 0.015 |
| $\tan(\cdot)$ | unary | yes | 0.015 |
| $\tanh(\cdot)$ | unary | yes | 0.015 |
| $\mathrm{atan}(\cdot)$ | unary | yes | 0.015 |
| $\cot(\cdot)$ | unary | yes | 0.015 |
| $\mathrm{acot}(\cdot)$ | unary | yes | 0.015 |
| $\csc(\cdot)$ | unary | yes | 0.015 |
| $\mathrm{sech}(\cdot)$ | unary | yes | 0.015 |
| $\mathrm{sinc}(\cdot)$ | unary | yes | 0.015 |
| $\lvert \cdot \rvert$ | unary | yes | 0.133 |
| $\sqrt{(\cdot)}$ | unary | yes | 0.133 |
| $(\cdot)^2$ | unary | yes | 0.133 |
| $(\cdot)^3$ | unary | yes | 0.133 |
| $\exp(\cdot)$ | unary | yes | 0.133 |
| $\log(\cdot)$ | unary | yes | 0.133 |
| $(\cdot) \times (\cdot)$ | binary | no | 0.8 |
| $^{(\cdot)}/_{(\cdot)}$ | binary | no | 0.2 |
| $(\cdot) + (\cdot)$ | binary | no | - |
| $\min(\cdot, \cdot)$ | binary | yes | 0.5 |
| $\max(\cdot, \cdot)$ | binary | yes | 0.5 |

Table A.2: Operators considered

| Explainer | | |
|---|---|---|
| LIME | num_samples | 5000 |
| | num_features | $d$ |
| | discretize_continuous | False |
| | feature_selection | 'auto' |
| MAPLE | train_size | 2/3 |
| | fe_type | 'rf' |
| | n_estimators | 200 |
| | max_features | 0.5 |
| | min_samples_leaf | 10 |
| | regularization | 1e-3 |
| SHAP | n_background_samples | 100 |
| | summarization | kmeans |
| | l1_reg | False |

Table A.3: Explainer hyperparameters

## Appendix B Proofs and Derivations

*Proof of* MATCHEFFECTS *Complexities*

The worst-case time complexity of MATCHEFFECTS is $\mathcal{O}\left(m_F m_{\hat{F}} d\right)$ and the space complexity is $\mathcal{O}\left(\max\left(d(m_F + m_{\hat{F}}), m_F m_{\hat{F}}\right)\right)$ (note that we write $\mathcal{O}\left(m_F m_{\hat{F}}\right)$ in the text for simplicity as the number of effects is almost always $\gg d$ in practical usage of the algorithm). Here we prove these claims, starting with the time complexity.

Lines 2-5 perform the following number of set intersections in the worst-case:

$$\begin{aligned} &\mathcal{O}(|D_F||D_{\hat{F}}|) \\ &= \mathcal{O}(m_F m_{\hat{F}}) \end{aligned}$$

Similarly, this is the worst-case number of edges $|E| = m_F m_{\hat{F}}$, which occurs if the bipartite graph is fully-connected (all effects relate to all other effects). Each set intersection (linear with hash sets in the implementation) has the following worst-case time complexity:

$$\begin{aligned} &\mathcal{O}\left(\max\left(\left\{|D_j| \mid D_j \in (D_F \cup D_{\hat{F}})\right\}\right)\right) \\ &= \mathcal{O}\left(|D_j^{\max}|\right) \\ &= \mathcal{O}\left(d\right) \end{aligned}$$

In the absolute worst-case every subset has $d$ features in the effect. Thus, the time complexity of these lines is $\mathcal{O}\left(m_F m_{\hat{F}} d\right)$.

In line 6, we compute the union of feature subsets (they become the graph vertices).

$$\begin{aligned} &\mathcal{O}\left(|V|\right) \\ &= \mathcal{O}\left(|D_F| + |D_{\hat{F}}|\right) \\ &= \mathcal{O}\left(m_F + m_{\hat{F}}\right) \end{aligned}$$

Set union takes linear time.

Line 8 performs the well-known connected components algorithm using graph traversal (BFS/DFS). Thus this takes

$$\begin{aligned} &\mathcal{O}(|V| + |E|) \\ &= \mathcal{O}\left(m_F + m_{\hat{F}} + m_F m_{\hat{F}}\right) \\ &= \mathcal{O}\left(m_F m_{\hat{F}}\right) \end{aligned}$$

time.

Lines 10-22 will traverse through each vertex exactly once (the vertices comprising each $V_c$ are guaranteed to be unique). For each vertex, checking membership in a set takes ($\mathcal{O}(1)$) time for each check. Thus, we have $\mathcal{O}(|V|) = \mathcal{O}\left(m_F + m_{\hat{F}}\right)$ for these lines. The match equality comparisons over all iterations in the loop will also take the same time per the guarantee each vertex is visited once.

Thus, the worst-case time complexity is $\mathcal{O}\left(m_F m_{\hat{F}} d\right)$ □

Here we consider the space complexity. The size of the graph is simply the size of the vertices and edges $\mathcal{O}(|V| + |E|) = \mathcal{O}\left(m_F m_{\hat{F}}\right)$. Note that the graph is represented in a sparse format (nonzero values only), though this doesn't reduce space in the dense worst-case scenario.

The other space to consider is from *matches*. This contains sets, each with two sets of effects (ground truth and explained). For efficiency, each effect is represented as an index, reducing the space required from $\mathcal{O}(d)$ to $\mathcal{O}(1)$. Thus *matches* ($|V|$ effects total, no matter how large a single match is) takes $\mathcal{O}(m_F + m_{\hat{F}})$ space.

Last, the input data is the same size as *matches*, except effects are not represented as indices. Therefore, the input data ($D_F$ and $D_{\hat{F}}$) takes $\mathcal{O}(d(m_F + m_{\hat{F}}))$ space.

The total space required is:

$\mathcal{O}\left(\max\left(d(m_F + m_{\hat{F}}), m_F m_{\hat{F}}\right)\right)$ □

*Derivation of Equivalence Relations*

*LIME*

For `LIME`, we derive the unnormalized coefficients for use in producing contributions. `LIME` uses z-score normalization ($(x_i - \mu_i)/\sigma_i$) on the input data before learning local linear regression models.

$$\hat{F}(\mathbf{x}) = \theta_0 + \sum_i^d \frac{x_i - \mu_i}{\sigma_i}\theta_i$$

$$\hat{F}(\mathbf{x}) = \theta_0 + \sum_i^d \left(\frac{x_i}{\sigma_i} - \frac{\mu_i}{\theta_i}\right)$$

$$\hat{F}(\mathbf{x}) = \left(\theta_0 - \frac{\mu_i}{\theta_i}\right) + \sum_i^d \frac{x_i}{\sigma_i}$$

Thus we simply just need to scale the coefficients as follows (same as the main text)

$$\theta_0' = \theta_0 - \sum_i \frac{\mu_i \theta_i}{\sigma_i}$$

$$\theta_i' = \frac{\theta_i}{\sigma_i}$$

where $\theta_0'$ is the adjusted bias term and each $\theta_i'$ is an adjusted coefficient.

*SHAP*

`SHAP` estimates the contributions relative to the mean-centered model response. In other words:

$$\hat{F}(\mathbf{X}) \approx F(\mathbf{X}) - \mathbb{E}\left[F(\mathbf{X})\right]$$

Thus, the `SHAP` estimation can be written as follows

$$\hat{F}(\mathbf{X}) = \sum_i^d \hat{f}_i\left(\mathbf{x}_{*,i}\right) - \mathbb{E}[f_i(\mathbf{x}_{*,i})]$$

due to the fact that

$$\begin{aligned}\mathbb{E}\left[F(\mathbf{X})\right] &= \mathbb{E}\left[\sum_{j}^{m} f_j\left(\mathbf{X}_{*,D_{f_j}}\right)\right] \\ &= \sum_{j}^{m} \mathbb{E}\left[f_j\left(\mathbf{X}_{*,D_{f_j}}\right)\right].\end{aligned}$$

So for each contribution, we can write that of the explainer as

$$C_{\hat{f}_i} = \hat{f}_i(\mathbf{x}_{*,i}) + \mathbb{E}[C_{f_i}]$$

in order to correct for the removed expected value. However, this assumes that there is some $i = j = k$ for every $f_j(\cdot)$ and $\hat{f}_k(\cdot)$ of the white box and explainer. As this is not always the case, we have to consider the effects of a match holistically. This then gives us the final relation for some match:

$$C_{match_{\hat{F}}} = \sum_{k \in match_{\hat{F}}} \hat{f}_k(\mathbf{x}_{*,k}) + \sum_{j \in match_F} \mathbb{E}[C_{f_j}]$$

This same process applies to `SHAPR`.

## Appendix C Additional Results and Figures

Table C.4 shows the MaIoU for each explainer on each dataset. Note that MaIoU is identical for both GAMs and NNs due to the experimental design: both are constrained to use the same (but still randomly selected) effects for each dataset. Of the explainers, `MAPLE` has the worst (lowest) average MaIoU due to its severe feature selection. *I.e.*, it picks relatively few features compared to the other explainers, which do not prune many by default. `LIME`, `SHAP`, and `SHAPR` achieve the same scores as they all provide feature-wise explanations and do not have feature selection enabled. This favors explanation completeness over human-comprehensibility, which is more favorable for testing fidelity. `PDP` follows the same line of reasoning except for FICO; `PDP` provides non-zero estimates of several more features than `LIME` and `SHAP` – recall that explanations of effects that are approximately zero are treated as a non-selected feature in our framework. On the MNIST task, all explainers achieve the same MaIoU, which seems counterintuitive at first. However, recall that in Appendix Appendix A under "Experiment Reproducibility" that the employed CNNs in effect operate on feature interactions of order two. Since the explainers in this experiment all provided feature-wise contributions, the MaIoU will always be 0.5 (assuming no feature selection). More concretely, each $E_c$ will comprise $\{\{\{D_{f_a}, D_{f_b}\}, \{D_{\hat{f}_i}\}\}, \{\{D_{f_a}, D_{f_b}\}, \{D_{\hat{f}_j}\}\}\}$. Assuming we have features '1' and '2' involved, we then have $E_c = \{\{\{1, 2\}, \{1\}\}, \{\{1, 2\}, \{2\}\}\}$. By definition aIoU is then $\frac{1}{2}(\frac{1}{2} + \frac{1}{2}) = 0.5$. As every $E_c$ will be of the same structure, aIoU will be the same and thus MaIoU is 0.5 by definition.

With the selection of nonlinear operators, more nonlinearities in models tend to drive the output range to somewhere within $[-1, 1]$. See Figures C.1 and C.2. For example, consider $\log(\tan(x))$ or $\sin(\max(x, 0))$. Thus, the absolute distance will likely decrease for all models with more nonlinearities. This is further compounded by the fact that explainers fail to explain models more often with more nonlinearities and features. What is interesting, however, is that `SHAP` improves in orientation with more nonlinearities whereas the other explainers

struggle. The Euclidean distance is again misleading here due to many models failed to be explained with more nonlinearities.

Figures are included that show examples of `SHAP` when it is relatively unfaithful, for instance Figures C.7 and C.8.

Figures C.10 through C.87 show the results on the real-world datasets for the GAMs and NNs. The local explanations over all instances (feature shapes) are illustrated for each individual feature, and captions give the NRMSE for pairwise effects and surrogate predictions. A subset of feature shapes is shown for the HELOC dataset due to the large number of features and the multiple classes. We also show the best and worst explanations per explainer on each dataset and model. This gives a great idea of how damaging an explanation could be to a user and how helpful it can be in understanding the local reasoning for a decision.

*More figures on the proceeding pages.*

| Dataset | MaIoU | | | | |
|---|---|---|---|---|---|
| | `PDP` | `LIME` | `MAPLE` | `SHAP` | `SHAPR` |
| Boston | 0.979 | 0.979 | 0.214 | 0.979 | 0.979 |
| COMPAS | 0.971 | 0.971 | 0.286 | 0.971 | – |
| FICO | 0.750 | 0.659 | 0.648 | 0.659 | – |
| MNIST | 0.500 | 0.500 | 0.500 | 0.500 | 0.500 |

Table C.4: The MaIoU for each explainer on several real-world datasets. Note that MaIoU is identical for both GAMs and NNs due to the experimental design: both are constrained to use the same (but still randomly selected) effects for each dataset. `SHAPR` is not implemented for data with categorical variables in this work.

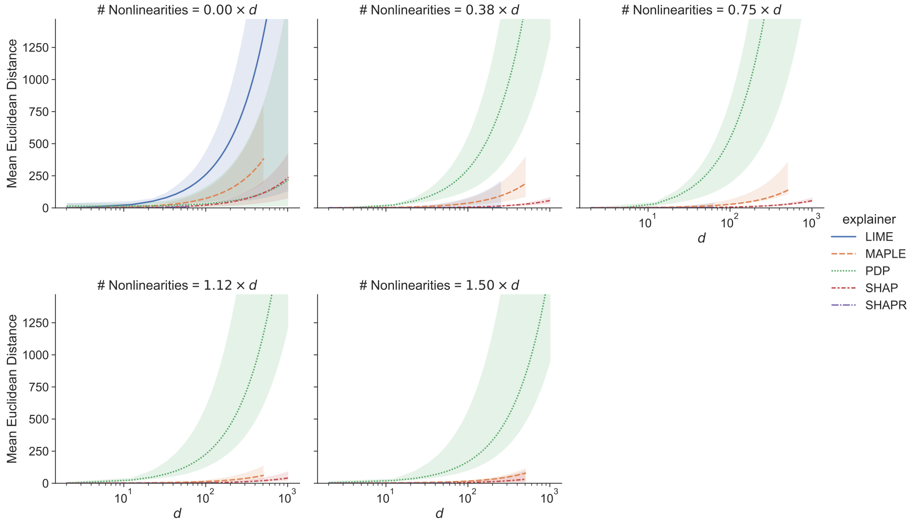


Figure C.1: Regression plots of Euclidean distance as a function of $d$ with each plot showing the ascending number of nonlinearities. See the main text for plotting details.

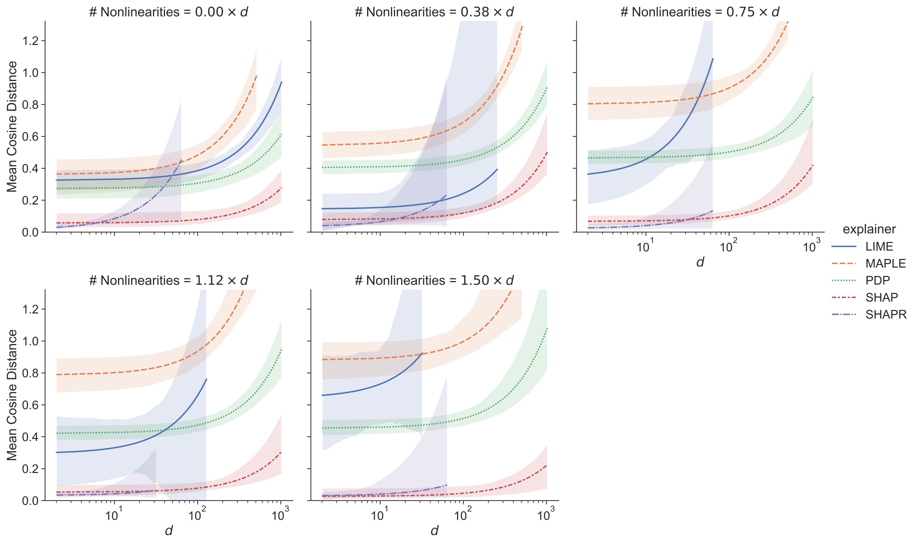


Figure C.2: Regression plots of cosine distance as a function of $d$ with each plot showing the ascending number of nonlinearities. See the main text for plotting details.

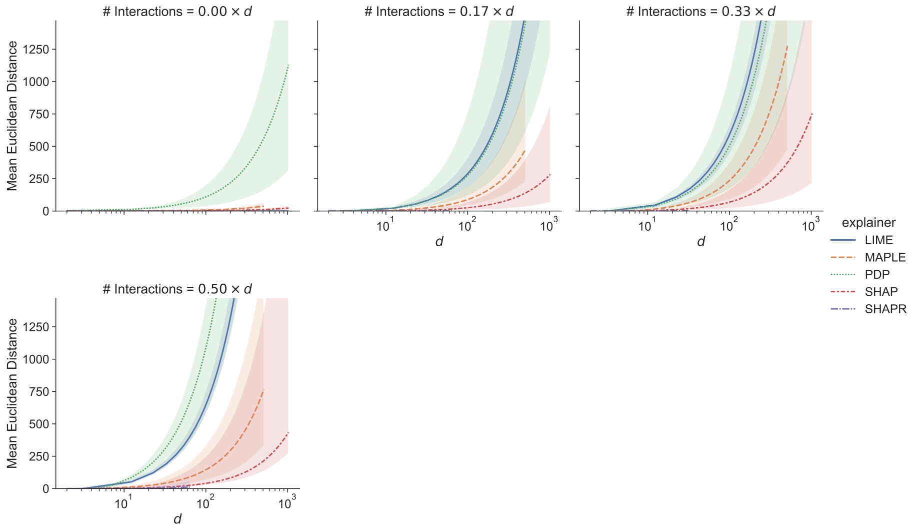


Figure C.3: Regression plots of Euclidean distance as a function of $d$ with each plot showing the ascending number of interaction terms. See the main text for plotting details.

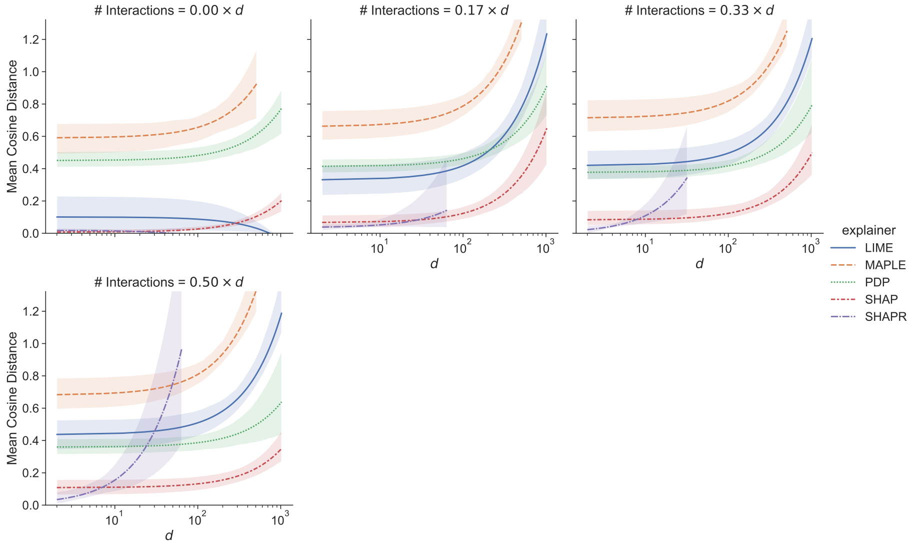


Figure C.4: Regression plots of cosine distance as a function of $d$ with each plot showing the ascending number of interaction terms. For the same reason mentioned in the main text, the top left plot of `LIME` is misleading here. See the main text for plotting details.

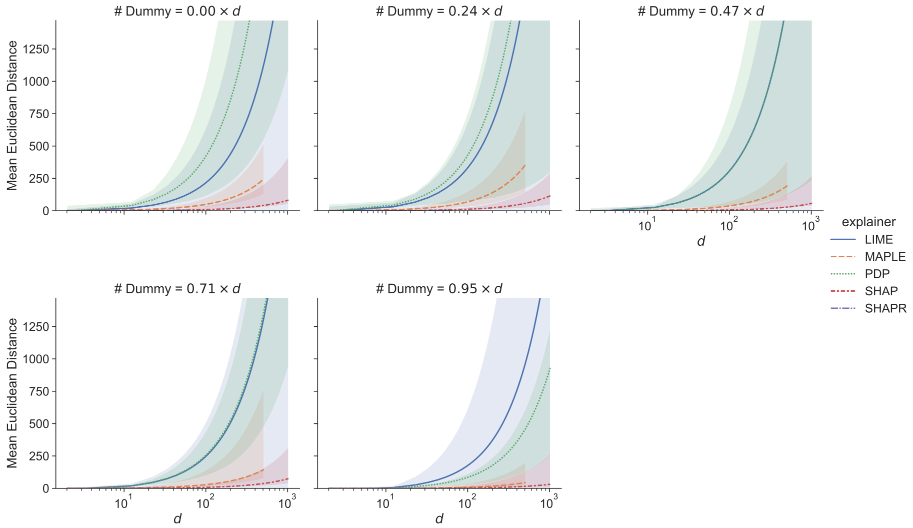


Figure C.5: Regression plots of Euclidean distance as a function of $d$ with each plot showing the ascending number of dummy features. See the main text for plotting details.

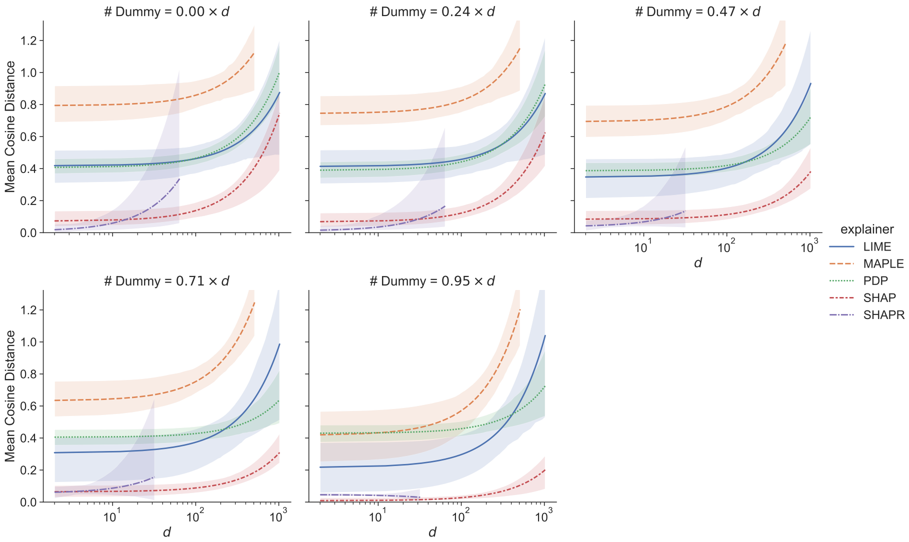


Figure C.6: Regression plots of cosine distance as a function of $d$ with each plot showing the ascending number of dummy features. See the main text for plotting details.

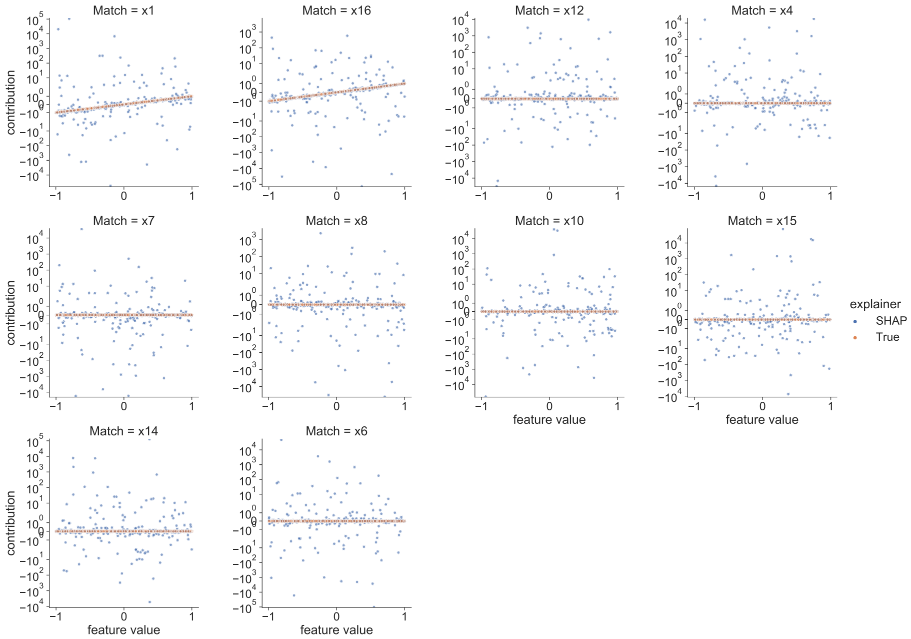


Figure C.7: Poor SHAP explanations for the randomly generated synthetic expression: $x_1 + \sqrt{x_{11}} + x_{13}x_2 + x_{13} + \frac{x_{13}}{\tanh(x_9)} + x_{16} + x_2x_9 + x_2 + x_3x_5 + x_3 + x_5^2 + e^{x_9} + \frac{x_2^3}{x_{11}^3}$. Features involved in interaction effects are not shown. Average cosine distance: 0.619. Average Euclidean distance: 2,890.

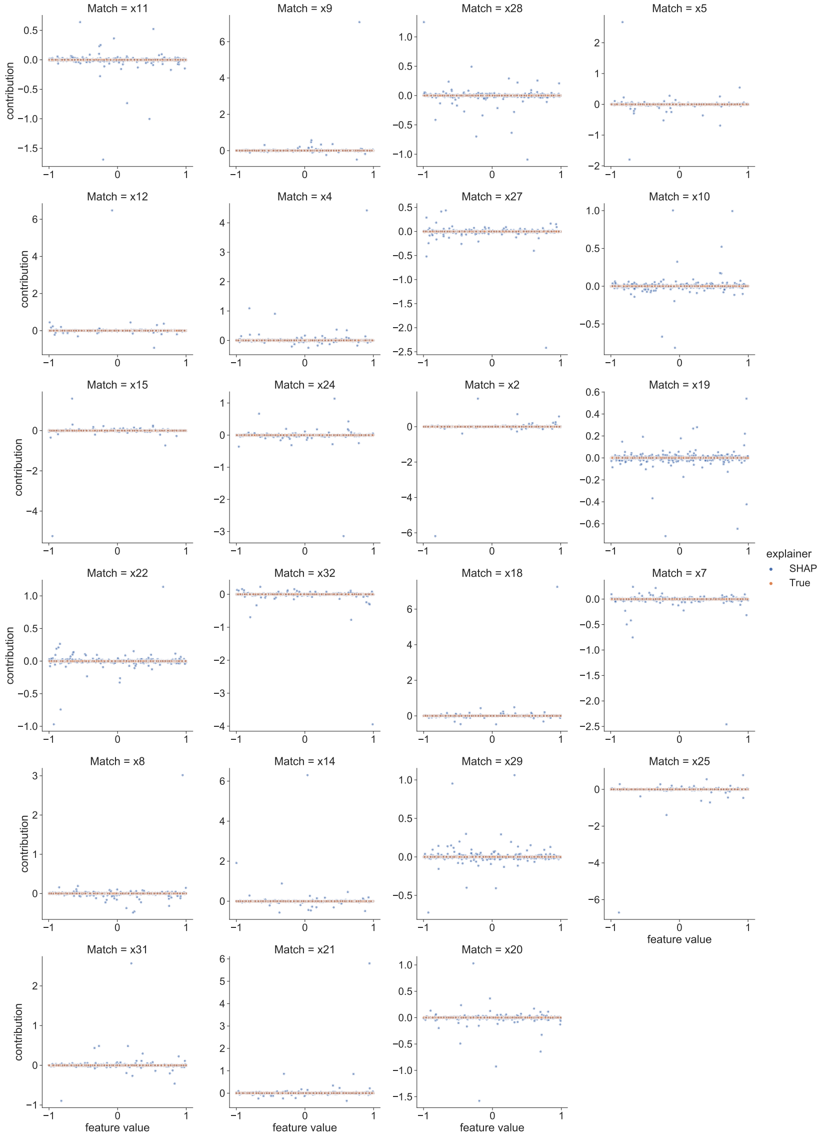


Figure C.8: Poor `SHAP` explanations for the randomly generated synthetic expression: $\frac{x_1^2}{x_{26}+x_3} + x_{17}^3 + x_{17}\left|x_1 + x_{30}\right| + x_{26}^3 + \frac{x_{26}}{\sqrt{x_1}+x_6} + x_3^3\left(x_{16}+x_6\right)^3 + x_3^2\left(x_{16}+x_{23}\right) + x_3\left(\begin{cases} x_1 & \text{for } x_1 < \left|x_{26}\right| \\ \left|x_{26}\right| & \text{otherwise} \end{cases}\right) + x_{30}^3 + x_6^3\left(x_{13}+x_{30}\right)^3 + \sqrt{x_{23}\left(x_{16}+x_{17}\right)} + \left(x_1 + x_{13}x_{30}\right)^3 + \left(x_{17}+x_{30}\right)\cot\left(x_1\right) + e^{x_{13}} + e^{x_3} + e^{x_6} + \tanh\left(x_{16}\right) + \left|x_1\right| + \left|x_{30}\left(x_1+x_{16}\right)\right| + \csc\left(x_{23}\right)$. Features involved in interaction effects are not shown. Average cosine distance: 1.21. Average Euclidean distance: 8.90.

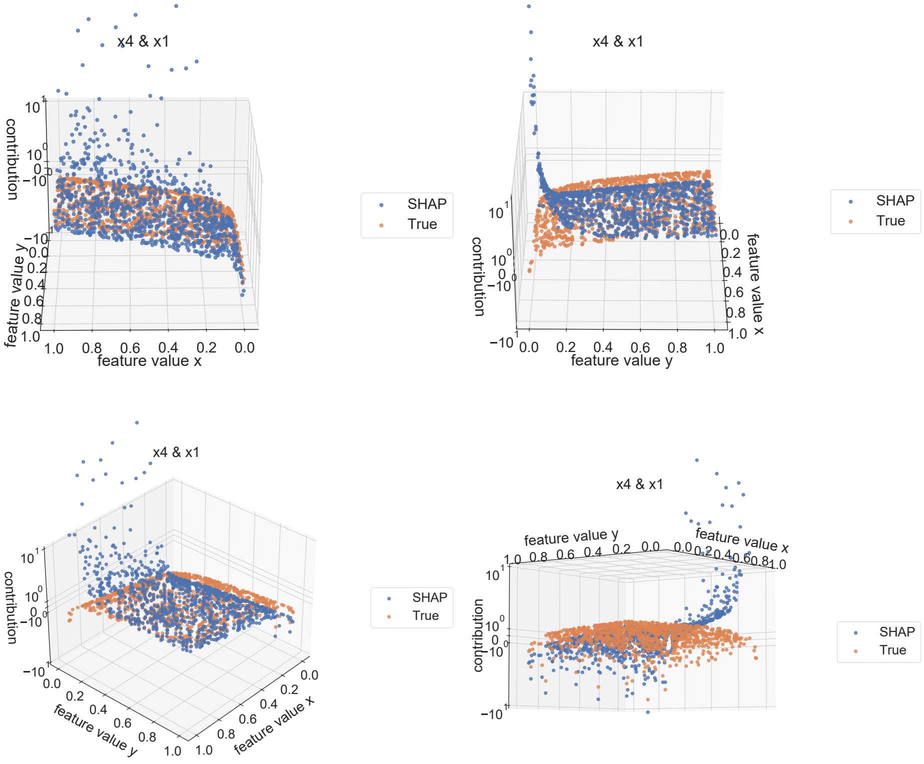


Figure C.9: Poor SHAP explanations for the randomly generated synthetic expression: $x_1 + e^{x_4} + \log(x_1 x_4) + \frac{x_4}{x_1}$. We show four different views of the same interaction term — with MatchEffects, every term of the expression is related to all of the explained variables, thus there is only one comparison made here. Average cosine distance: 0.492. Average Euclidean distance: 2.54.

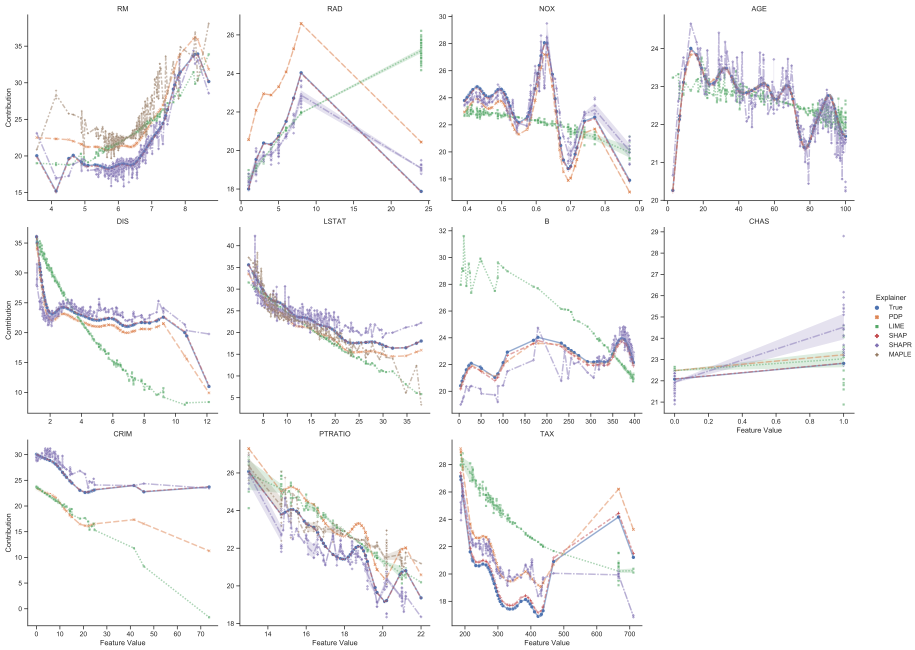


Figure C.10: Feature shapes of the main effects of a GAM that was trained on the Boston Housing dataset and the explainers. The subtitle indicates the feature name. Median NRMSE scores over all effects: 0.709 (`LIME`), 0.652 (`MAPLE`), 0.340 (`PDP`), 0.001 (`SHAP`), 0.111 (`SHAPR`).

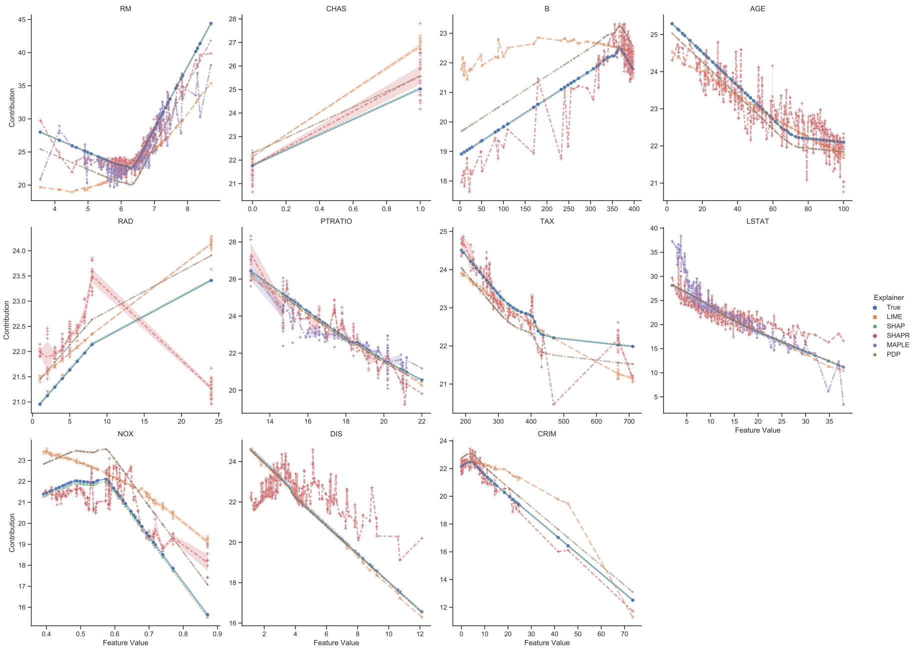


Figure C.11: Feature shapes of the main effects of a NN that was trained on the Boston Housing dataset and the explainers. The subtitle indicates the feature name. Median NRMSE scores over all effects: 0.182 (**LIME**), 0.431 (**MAPLE**), 0.278 (**PDP**), 0.001 (**SHAP**), 0.209 (**SHAPR**).

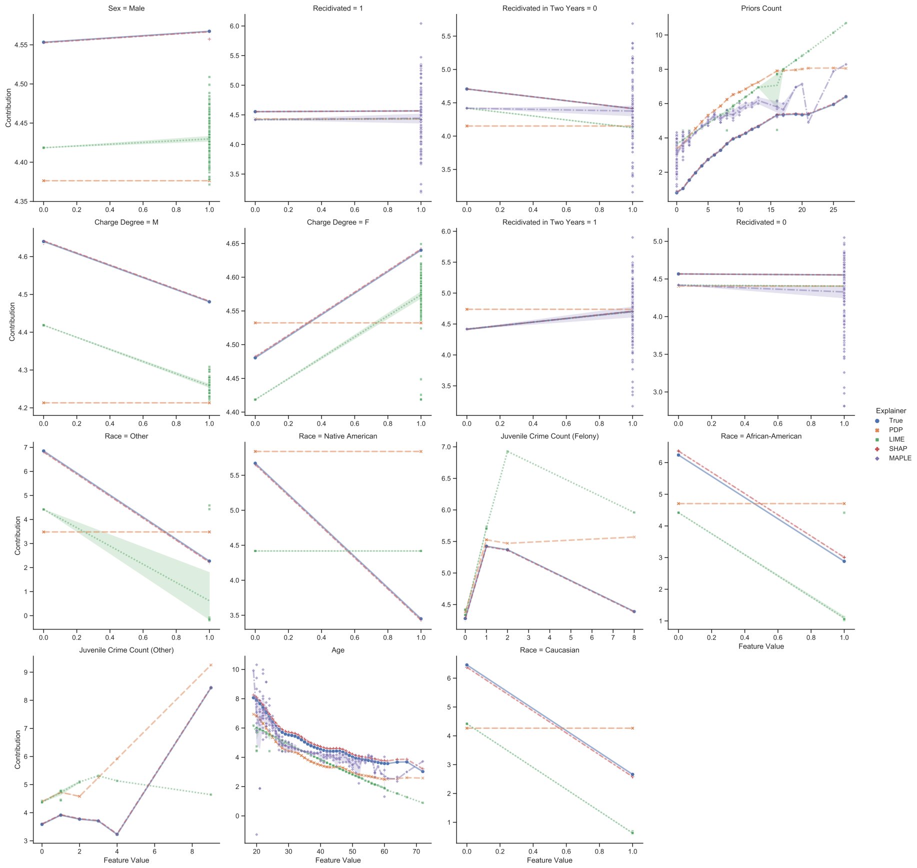


Figure C.12: Feature shapes of the main effects of a GAM that was trained on the COMPAS dataset and the explainers. The subtitle indicates the feature name. Median NRMSE scores over all effects: 0.781 (`LIME`), 0.863 (`MAPLE`), 0.821 (`PDP`), 0.000 (`SHAP`).

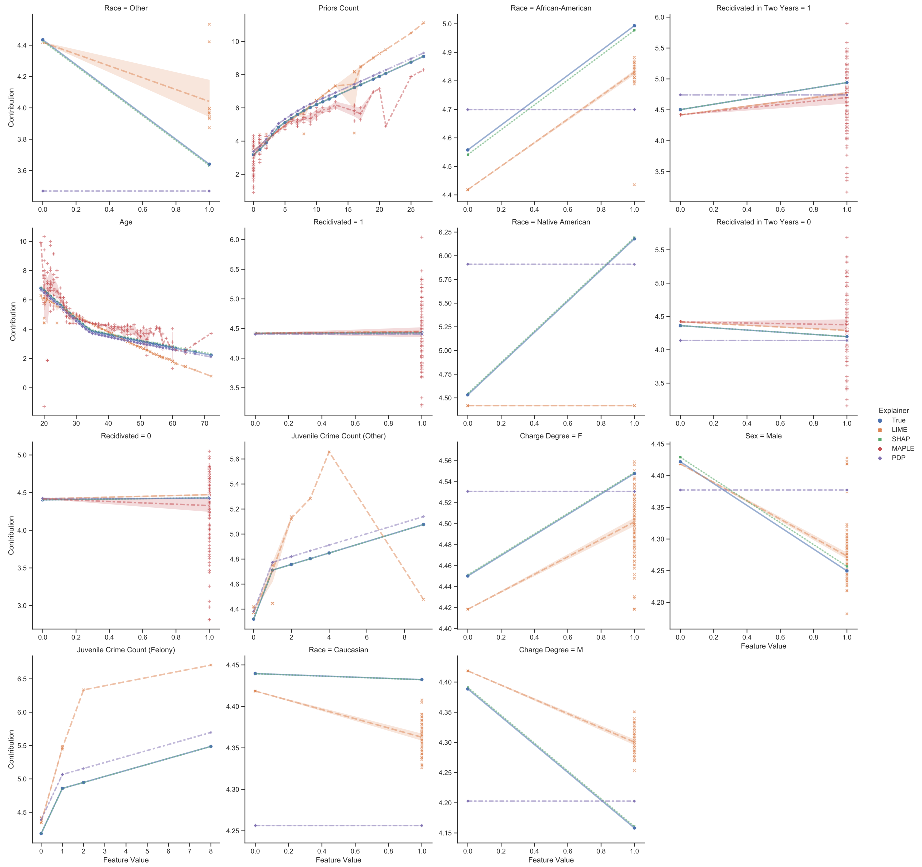


Figure C.13: Feature shapes of the main effects of a NN that was trained on the COMPAS dataset and the explainers. The subtitle indicates the feature name. Median NRMSE scores over all effects: 0.062 (`LIME`), 0.274 (`MAPLE`), 0.328 (`PDP`), 0.001 (`SHAP`).

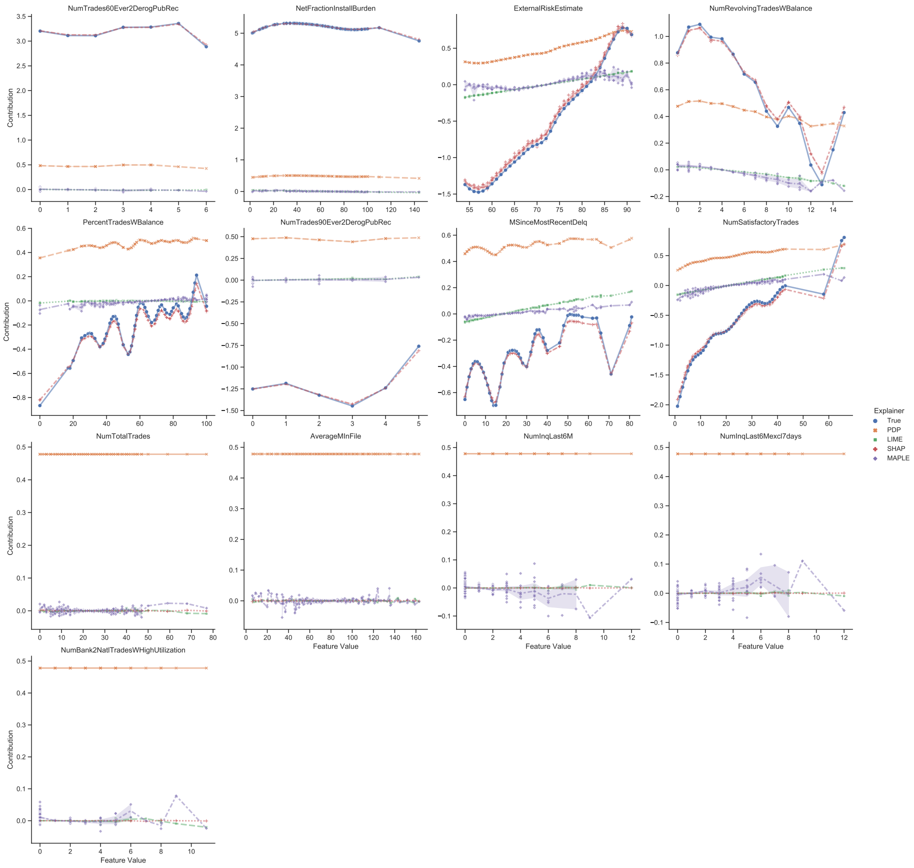


Figure C.14: Feature shapes of the main effects of a GAM that was trained on the HELOC dataset and the explainers. The subtitle indicates the feature name. Median NRMSE scores over all effects: 0.949 (`LIME`), 0.963 (`MAPLE`), 0.795 (`PDP`), 0.003 (`SHAP`).

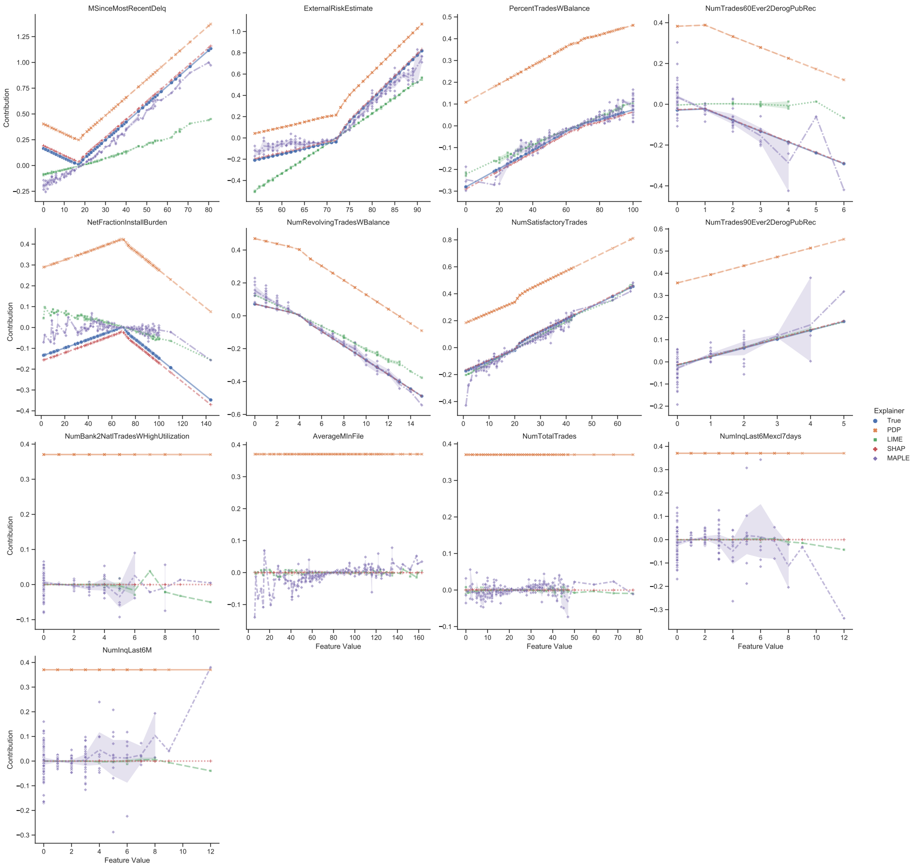


Figure C.15: Feature shapes of the main effects of a GAM that was trained on the HELOC dataset and the explainers. The subtitle indicates the feature name. Median NRMSE scores over all effects: 0.193 (**LIME**), 0.226 (**MAPLE**), 0.761 (**PDP**), 0.010 (**SHAP**).

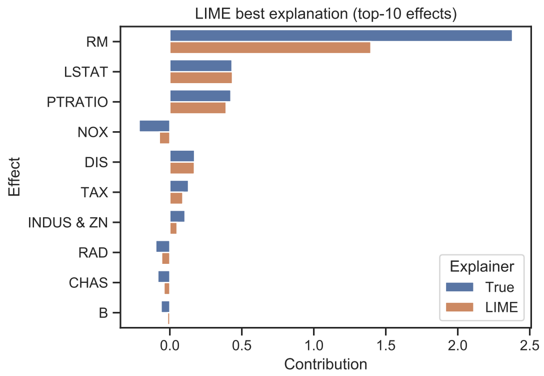


Figure C.16: The top-10 explained effects of the best explanation by `LIME` for a DNN trained on the Boston dataset. Top effects are ranked by magnitude and the quality of explanation is ranked by mean cosine distance among all explained samples.

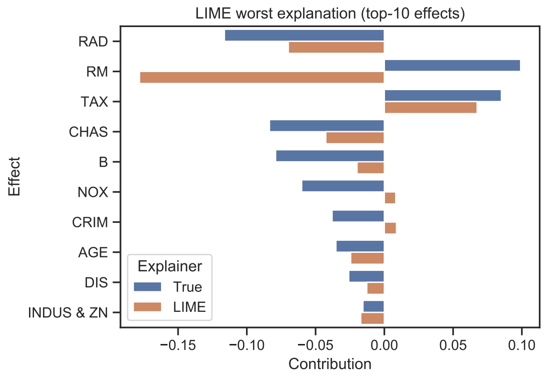


Figure C.17: The top-10 explained effects of the worst explanation by `LIME` for a DNN trained on the Boston dataset. Top effects are ranked by magnitude and the quality of explanation is ranked by mean cosine distance among all explained samples.

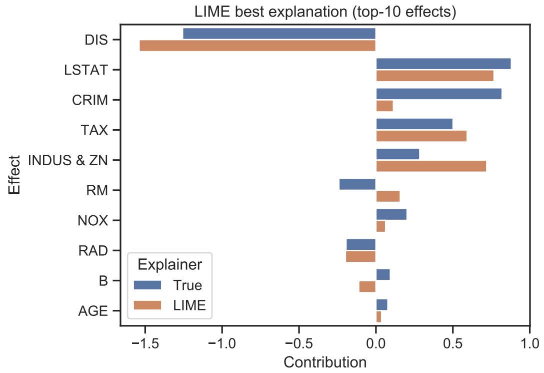


Figure C.18: The top-10 explained effects of the best explanation by `LIME` for a GAM trained on the Boston dataset. Top effects are ranked by magnitude and the quality of explanation is ranked by mean cosine distance among all explained samples.

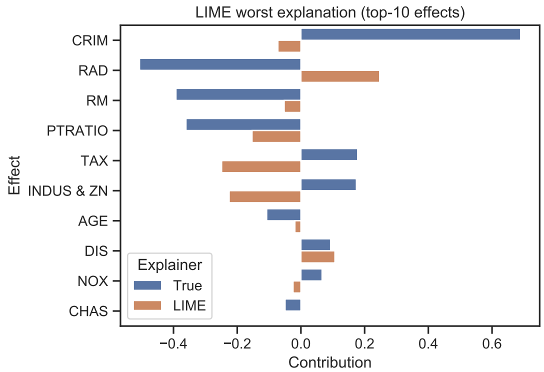


Figure C.19: The top-10 explained effects of the worst explanation by `LIME` for a GAM trained on the Boston dataset. Top effects are ranked by magnitude and the quality of explanation is ranked by mean cosine distance among all explained samples.

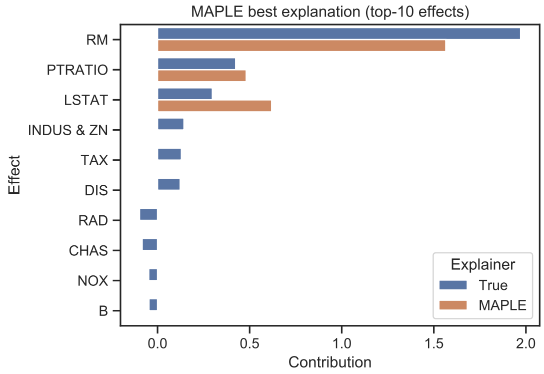


Figure C.20: The top-10 explained effects of the best explanation by `MAPLE` for a DNN trained on the Boston dataset. Top effects are ranked by magnitude and the quality of explanation is ranked by mean cosine distance among all explained samples.

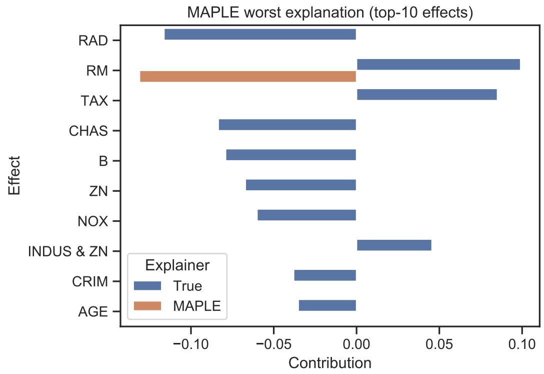


Figure C.21: The top-10 explained effects of the worst explanation by `MAPLE` for a DNN trained on the Boston dataset. Top effects are ranked by magnitude and the quality of explanation is ranked by mean cosine distance among all explained samples.

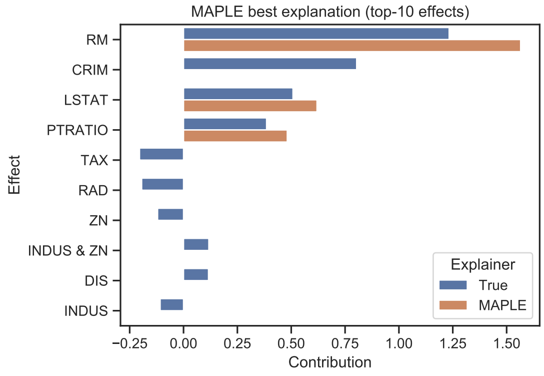


Figure C.22: The top-10 explained effects of the best explanation by `MAPLE` for a GAM trained on the Boston dataset. Top effects are ranked by magnitude and the quality of explanation is ranked by mean cosine distance among all explained samples.

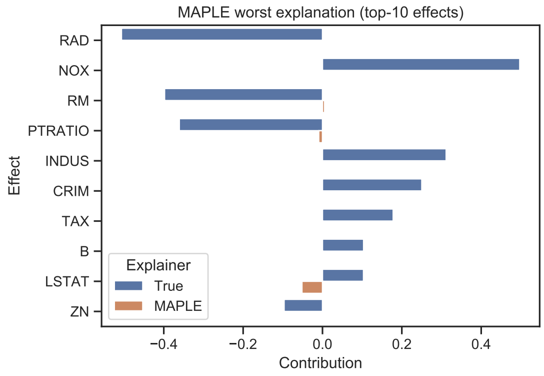


Figure C.23: The top-10 explained effects of the worst explanation by `MAPLE` for a GAM trained on the Boston dataset. Top effects are ranked by magnitude and the quality of explanation is ranked by mean cosine distance among all explained samples.

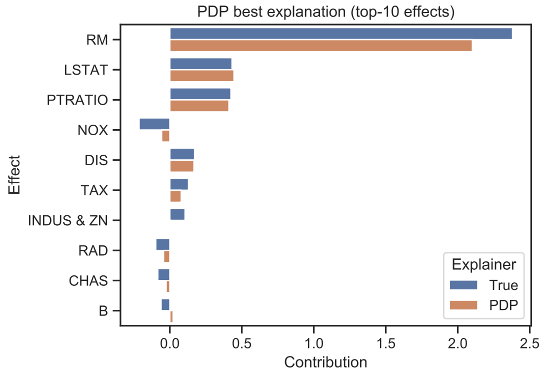


Figure C.24: The top-10 explained effects of the best explanation by `PDP` for a DNN trained on the Boston dataset. Top effects are ranked by magnitude and the quality of explanation is ranked by mean cosine distance among all explained samples.

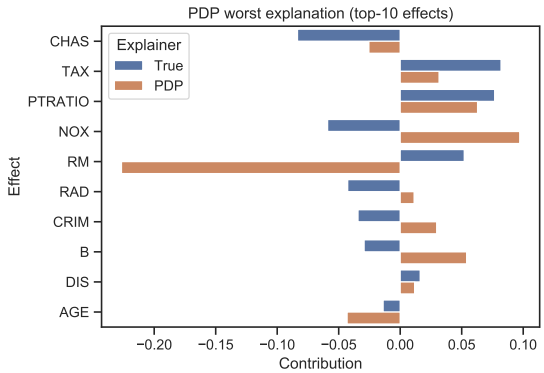


Figure C.25: The top-10 explained effects of the worst explanation by `PDP` for a DNN trained on the Boston dataset. Top effects are ranked by magnitude and the quality of explanation is ranked by mean cosine distance among all explained samples.

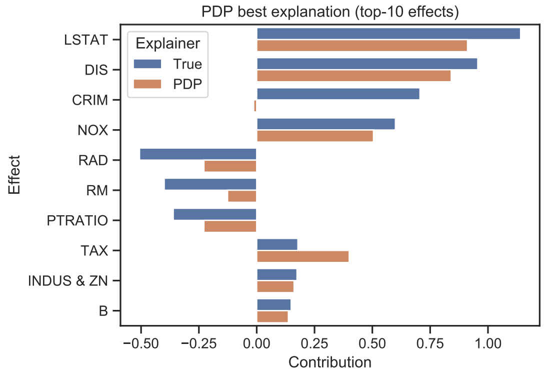


Figure C.26: The top-10 explained effects of the best explanation by `PDP` for a GAM trained on the Boston dataset. Top effects are ranked by magnitude and the quality of explanation is ranked by mean cosine distance among all explained samples.

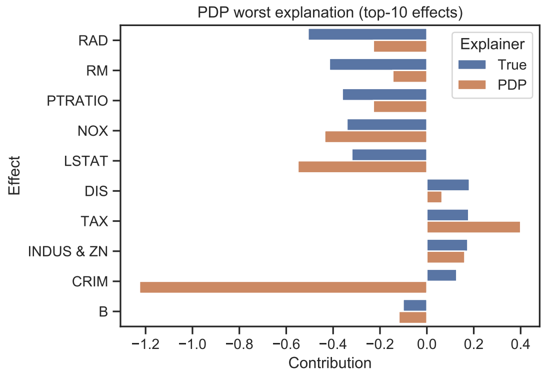


Figure C.27: The top-10 explained effects of the worst explanation by `PDP` for a GAM trained on the Boston dataset. Top effects are ranked by magnitude and the quality of explanation is ranked by mean cosine distance among all explained samples.

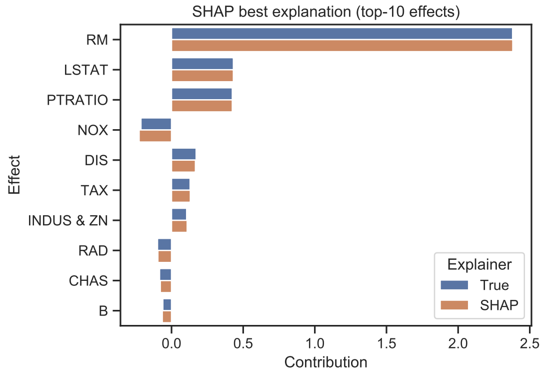


Figure C.28: The top-10 explained effects of the best explanation by `SHAP` for a DNN trained on the Boston dataset. Top effects are ranked by magnitude and the quality of explanation is ranked by mean cosine distance among all explained samples.

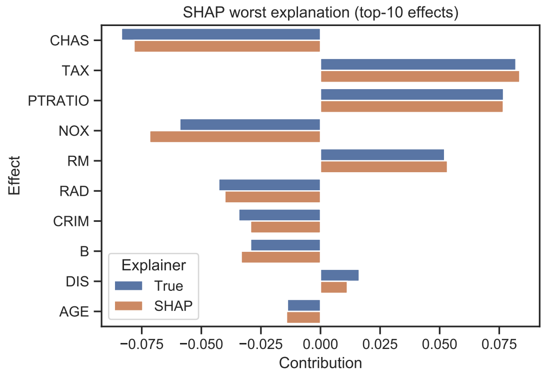


Figure C.29: The top-10 explained effects of the worst explanation by `SHAP` for a DNN trained on the Boston dataset. Top effects are ranked by magnitude and the quality of explanation is ranked by mean cosine distance among all explained samples.

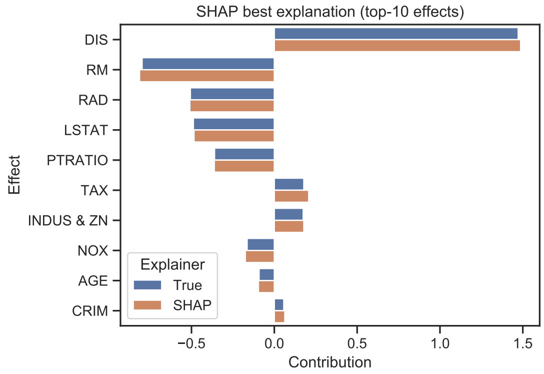


Figure C.30: The top-10 explained effects of the best explanation by `SHAP` for a GAM trained on the Boston dataset. Top effects are ranked by magnitude and the quality of explanation is ranked by mean cosine distance among all explained samples.

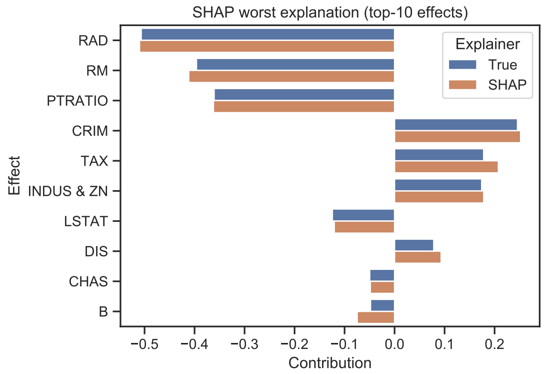


Figure C.31: The top-10 explained effects of the worst explanation by `SHAP` for a GAM trained on the Boston dataset. Top effects are ranked by magnitude and the quality of explanation is ranked by mean cosine distance among all explained samples.

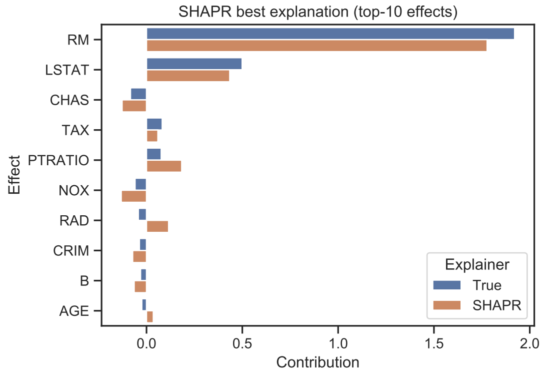


Figure C.32: The top-10 explained effects of the best explanation by **SHAPR** for a DNN trained on the Boston dataset. Top effects are ranked by magnitude and the quality of explanation is ranked by mean cosine distance among all explained samples.

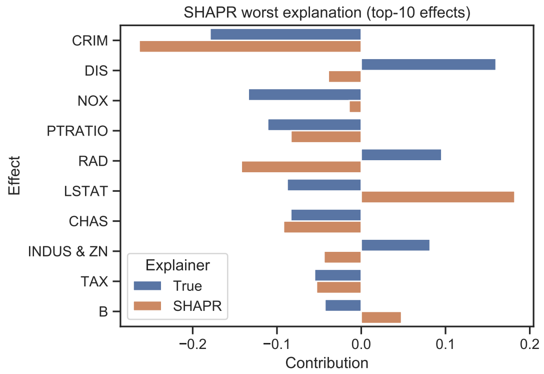


Figure C.33: The top-10 explained effects of the worst explanation by **SHAPR** for a DNN trained on the Boston dataset. Top effects are ranked by magnitude and the quality of explanation is ranked by mean cosine distance among all explained samples.

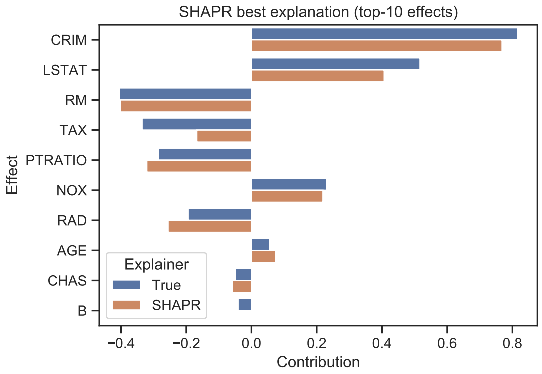


Figure C.34: The top-10 explained effects of the best explanation by `SHAPR` for a GAM trained on the Boston dataset. Top effects are ranked by magnitude and the quality of explanation is ranked by mean cosine distance among all explained samples.

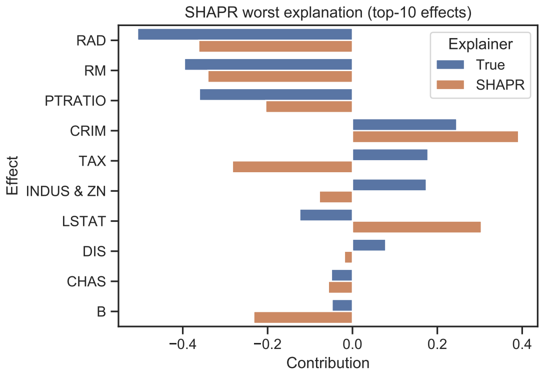


Figure C.35: The top-10 explained effects of the worst explanation by `SHAPR` for a GAM trained on the Boston dataset. Top effects are ranked by magnitude and the quality of explanation is ranked by mean cosine distance among all explained samples.

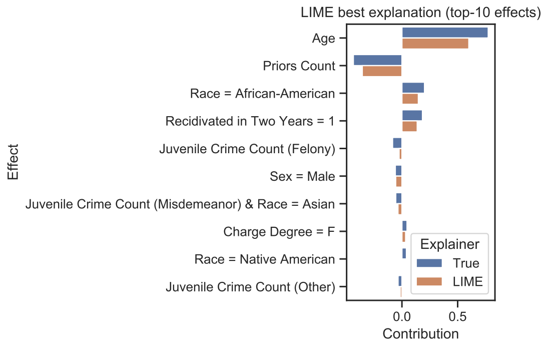


Figure C.36: The top-10 explained effects of the best explanation by `LIME` for a DNN trained on the COMPAS dataset. Top effects are ranked by magnitude and the quality of explanation is ranked by mean cosine distance among all explained samples.

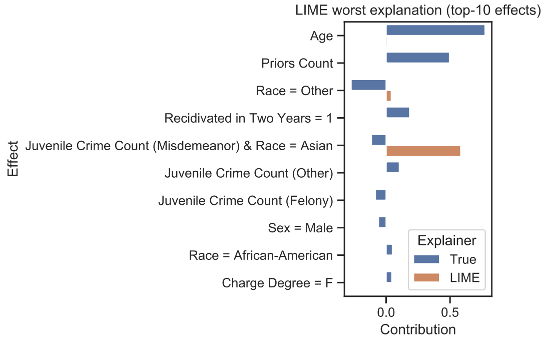


Figure C.37: The top-10 explained effects of the worst explanation by `LIME` for a DNN trained on the COMPAS dataset. Top effects are ranked by magnitude and the quality of explanation is ranked by mean cosine distance among all explained samples.

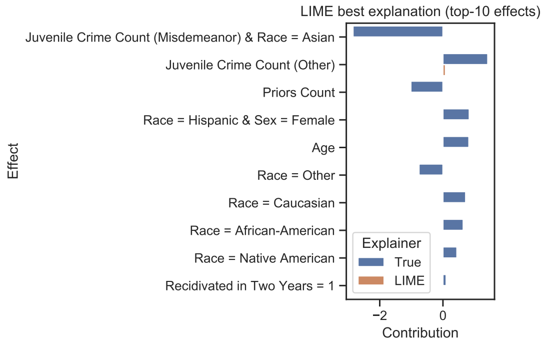


Figure C.38: The top-10 explained effects of the best explanation by `LIME` for a GAM trained on the COMPAS dataset. Top effects are ranked by magnitude and the quality of explanation is ranked by mean cosine distance among all explained samples.

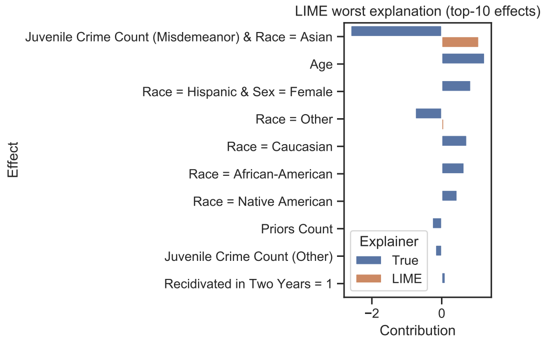


Figure C.39: The top-10 explained effects of the worst explanation by `LIME` for a GAM trained on the COMPAS dataset. Top effects are ranked by magnitude and the quality of explanation is ranked by mean cosine distance among all explained samples.

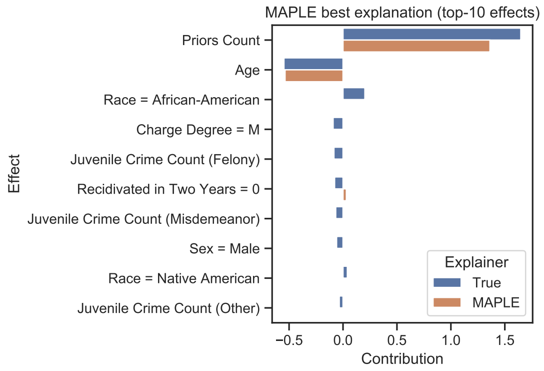


Figure C.40: The top-10 explained effects of the best explanation by `MAPLE` for a DNN trained on the COMPAS dataset. Top effects are ranked by magnitude and the quality of explanation is ranked by mean cosine distance among all explained samples.

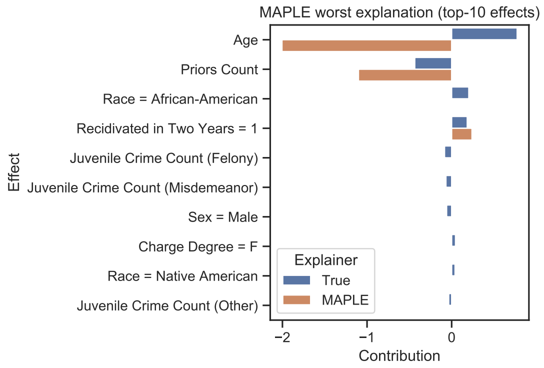


Figure C.41: The top-10 explained effects of the worst explanation by `MAPLE` for a DNN trained on the COMPAS dataset. Top effects are ranked by magnitude and the quality of explanation is ranked by mean cosine distance among all explained samples.

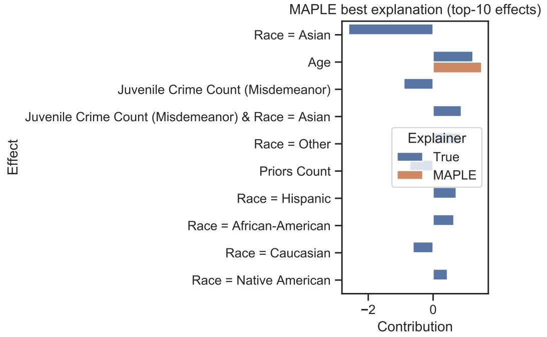


Figure C.42: The top-10 explained effects of the best explanation by `MAPLE` for a GAM trained on the COMPAS dataset. Top effects are ranked by magnitude and the quality of explanation is ranked by mean cosine distance among all explained samples.

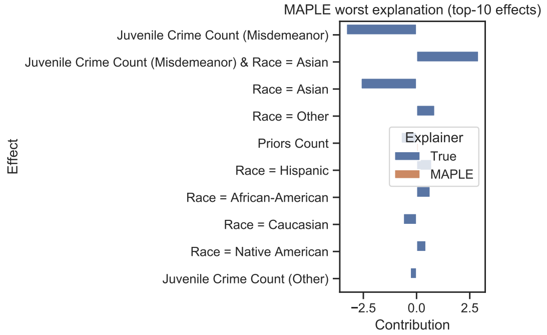


Figure C.43: The top-10 explained effects of the worst explanation by `MAPLE` for a GAM trained on the COMPAS dataset. Top effects are ranked by magnitude and the quality of explanation is ranked by mean cosine distance among all explained samples.

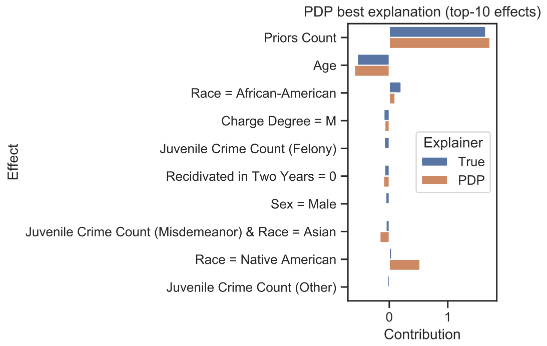


Figure C.44: The top-10 explained effects of the best explanation by PDP for a DNN trained on the COMPAS dataset. Top effects are ranked by magnitude and the quality of explanation is ranked by mean cosine distance among all explained samples.

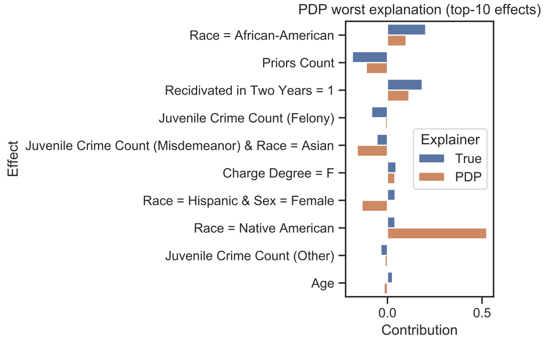


Figure C.45: The top-10 explained effects of the worst explanation by PDP for a DNN trained on the COMPAS dataset. Top effects are ranked by magnitude and the quality of explanation is ranked by mean cosine distance among all explained samples.

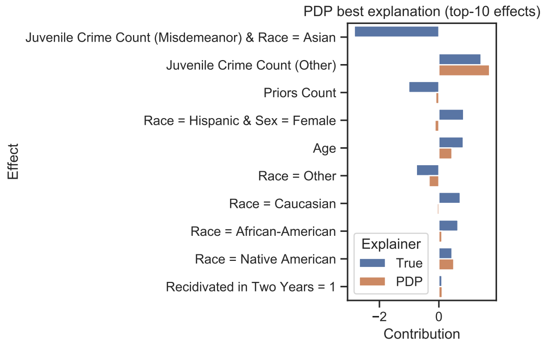


Figure C.46: The top-10 explained effects of the best explanation by `PDP` for a GAM trained on the COMPAS dataset. Top effects are ranked by magnitude and the quality of explanation is ranked by mean cosine distance among all explained samples.

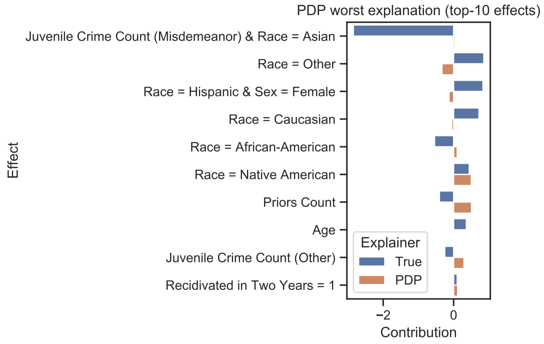


Figure C.47: The top-10 explained effects of the worst explanation by `PDP` for a GAM trained on the COMPAS dataset. Top effects are ranked by magnitude and the quality of explanation is ranked by mean cosine distance among all explained samples.

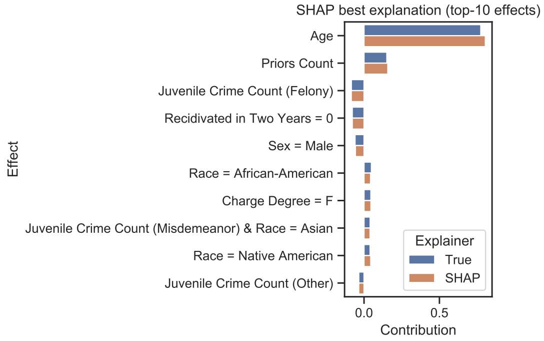


Figure C.48: The top-10 explained effects of the best explanation by `SHAP` for a DNN trained on the COMPAS dataset. Top effects are ranked by magnitude and the quality of explanation is ranked by mean cosine distance among all explained samples.

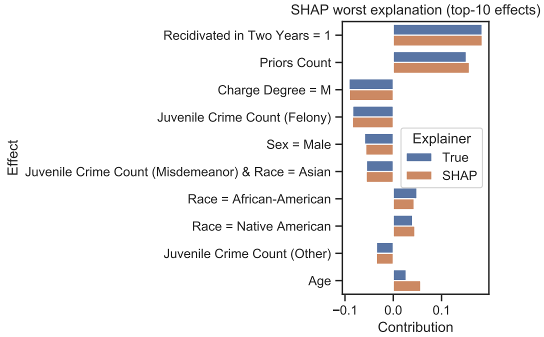


Figure C.49: The top-10 explained effects of the worst explanation by `SHAP` for a DNN trained on the COMPAS dataset. Top effects are ranked by magnitude and the quality of explanation is ranked by mean cosine distance among all explained samples.

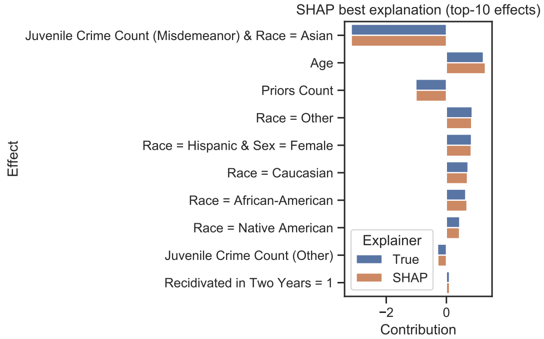


Figure C.50: The top-10 explained effects of the best explanation by `SHAP` for a GAM trained on the COMPAS dataset. Top effects are ranked by magnitude and the quality of explanation is ranked by mean cosine distance among all explained samples.

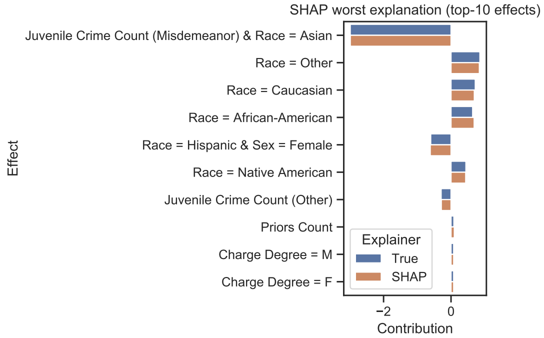


Figure C.51: The top-10 explained effects of the worst explanation by `SHAP` for a GAM trained on the COMPAS dataset. Top effects are ranked by magnitude and the quality of explanation is ranked by mean cosine distance among all explained samples.

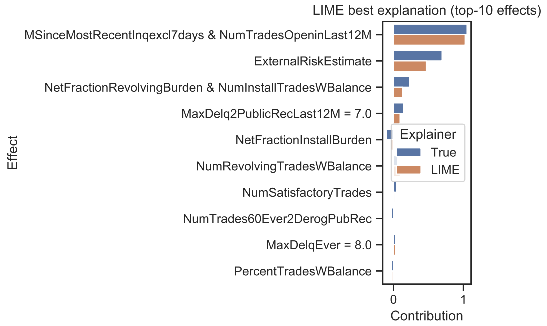


Figure C.52: The top-10 explained effects of the best explanation by `LIME` for a DNN trained on the FICO HELOC dataset. Top effects are ranked by magnitude and the quality of explanation is ranked by mean cosine distance among all explained samples.

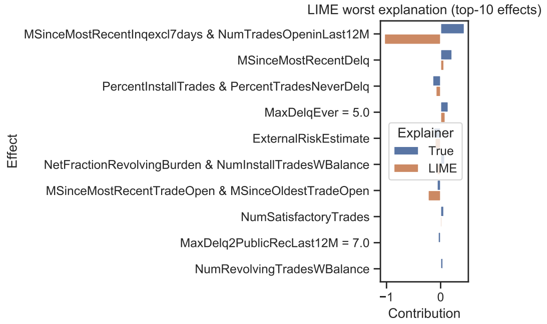


Figure C.53: The top-10 explained effects of the worst explanation by `LIME` for a DNN trained on the FICO HELOC dataset. Top effects are ranked by magnitude and the quality of explanation is ranked by mean cosine distance among all explained samples.

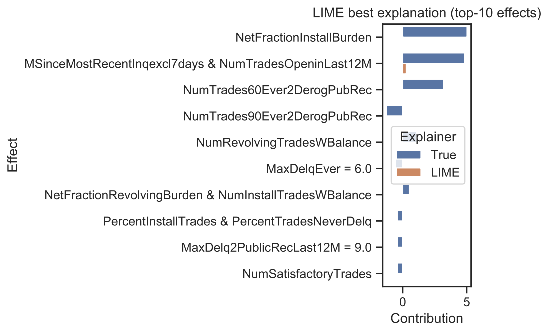


Figure C.54: The top-10 explained effects of the best explanation by `LIME` for a GAM trained on the FICO HELOC dataset. Top effects are ranked by magnitude and the quality of explanation is ranked by mean cosine distance among all explained samples.

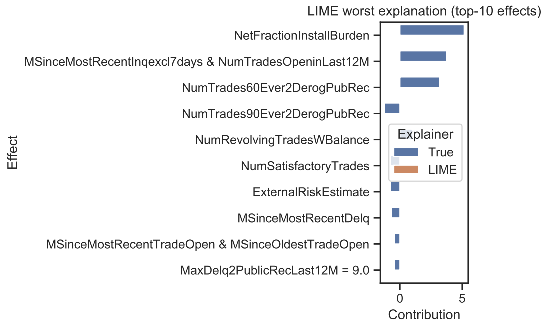


Figure C.55: The top-10 explained effects of the worst explanation by `LIME` for a GAM trained on the FICO HELOC dataset. Top effects are ranked by magnitude and the quality of explanation is ranked by mean cosine distance among all explained samples.

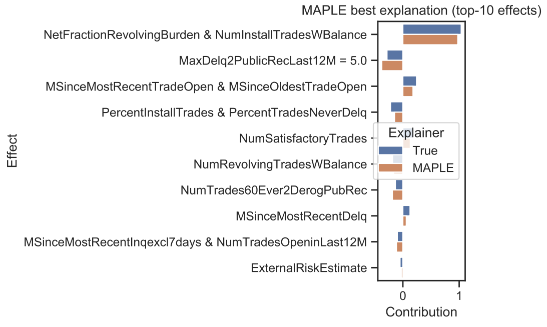


Figure C.56: The top-10 explained effects of the best explanation by `MAPLE` for a DNN trained on the FICO HELOC dataset. Top effects are ranked by magnitude and the quality of explanation is ranked by mean cosine distance among all explained samples.

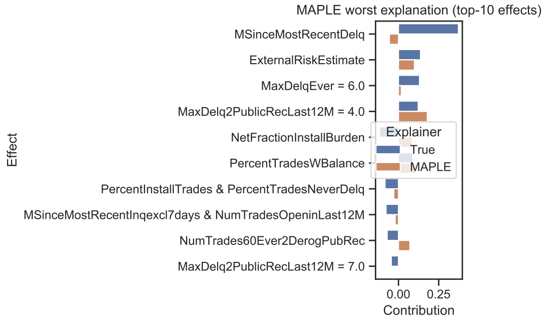


Figure C.57: The top-10 explained effects of the worst explanation by `MAPLE` for a DNN trained on the FICO HELOC dataset. Top effects are ranked by magnitude and the quality of explanation is ranked by mean cosine distance among all explained samples.

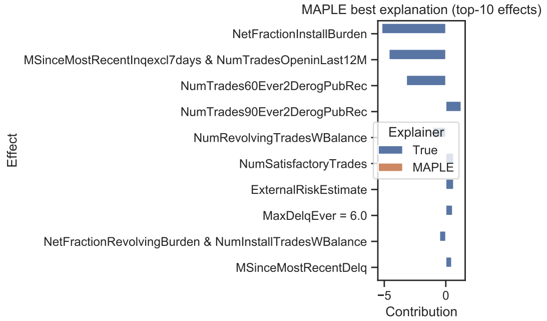


Figure C.58: The top-10 explained effects of the best explanation by `MAPLE` for a GAM trained on the FICO HELOC dataset. Top effects are ranked by magnitude and the quality of explanation is ranked by mean cosine distance among all explained samples.

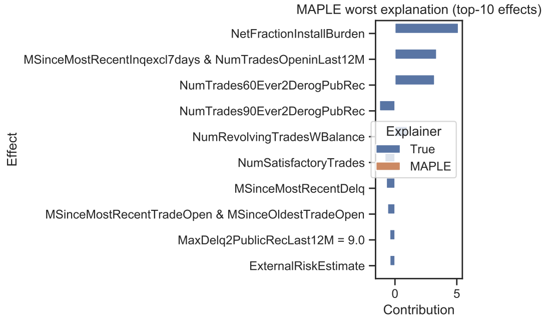


Figure C.59: The top-10 explained effects of the worst explanation by `MAPLE` for a GAM trained on the FICO HELOC dataset. Top effects are ranked by magnitude and the quality of explanation is ranked by mean cosine distance among all explained samples.

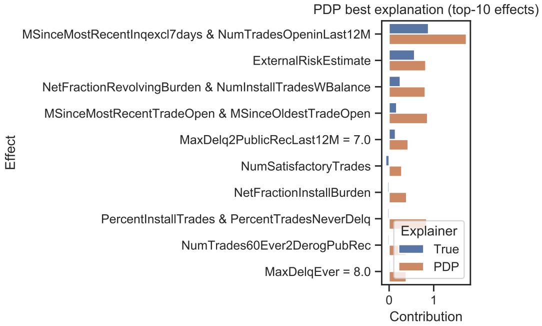


Figure C.60: The top-10 explained effects of the best explanation by PDP for a DNN trained on the FICO HELOC dataset. Top effects are ranked by magnitude and the quality of explanation is ranked by mean cosine distance among all explained samples.

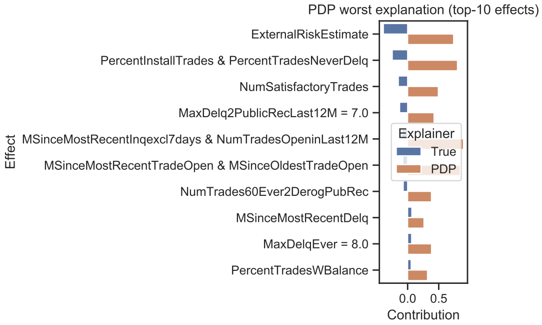


Figure C.61: The top-10 explained effects of the worst explanation by PDP for a DNN trained on the FICO HELOC dataset. Top effects are ranked by magnitude and the quality of explanation is ranked by mean cosine distance among all explained samples.

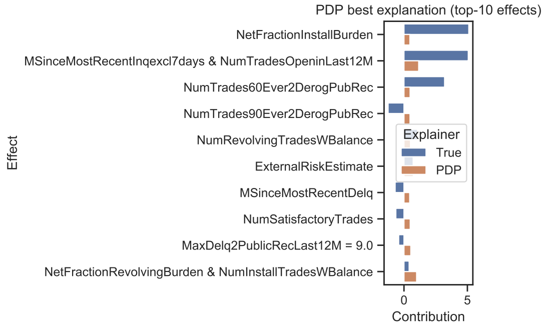


Figure C.62: The top-10 explained effects of the best explanation by PDP for a GAM trained on the FICO HELOC dataset. Top effects are ranked by magnitude and the quality of explanation is ranked by mean cosine distance among all explained samples.

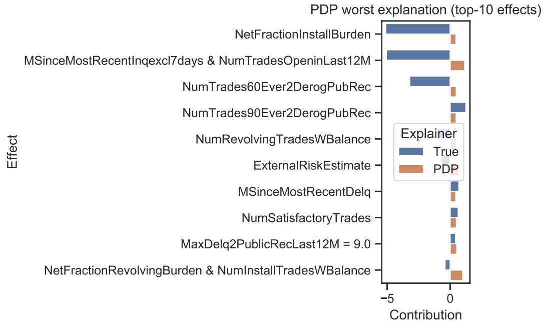


Figure C.63: The top-10 explained effects of the worst explanation by PDP for a GAM trained on the FICO HELOC dataset. Top effects are ranked by magnitude and the quality of explanation is ranked by mean cosine distance among all explained samples.

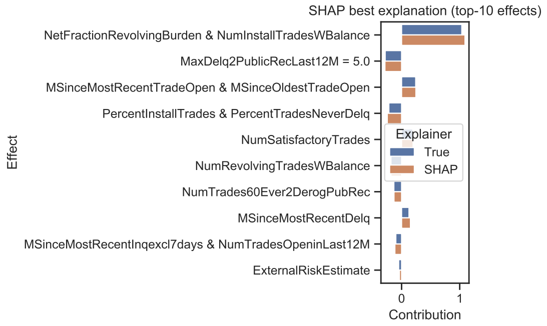


Figure C.64: The top-10 explained effects of the best explanation by `SHAP` for a DNN trained on the FICO HELOC dataset. Top effects are ranked by magnitude and the quality of explanation is ranked by mean cosine distance among all explained samples.

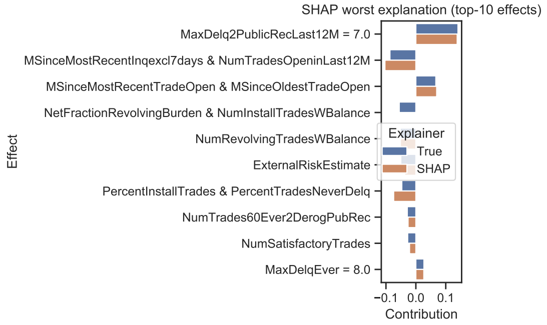


Figure C.65: The top-10 explained effects of the worst explanation by `SHAP` for a DNN trained on the FICO HELOC dataset. Top effects are ranked by magnitude and the quality of explanation is ranked by mean cosine distance among all explained samples.

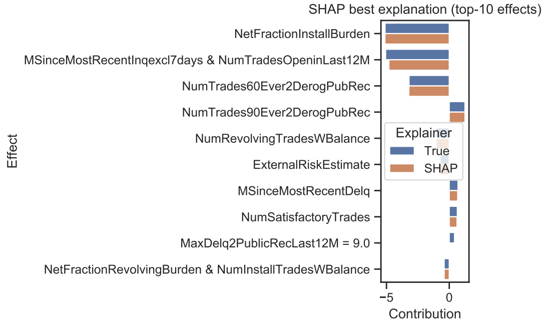


Figure C.66: The top-10 explained effects of the best explanation by `SHAP` for a GAM trained on the FICO HELOC dataset. Top effects are ranked by magnitude and the quality of explanation is ranked by mean cosine distance among all explained samples.

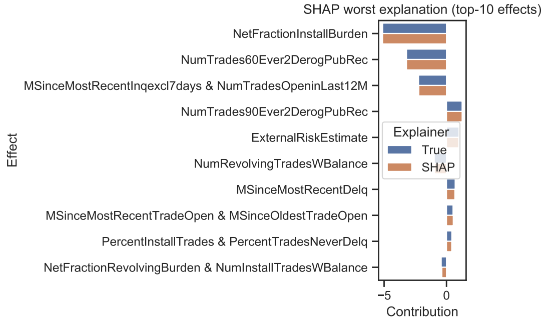


Figure C.67: The top-10 explained effects of the worst explanation by `SHAP` for a GAM trained on the FICO HELOC dataset. Top effects are ranked by magnitude and the quality of explanation is ranked by mean cosine distance among all explained samples.

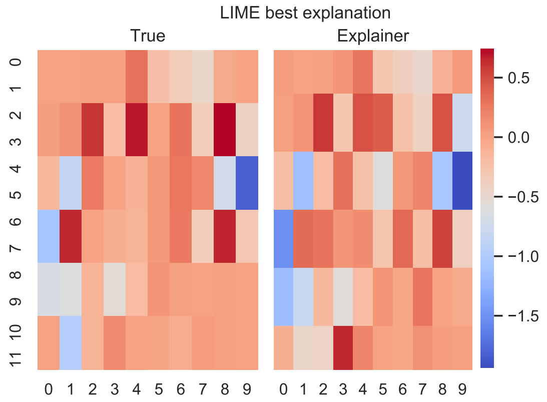


Figure C.68: The heatmap of explained effects of the best explanation by `LIME` for a CNN trained on the MNIST dataset.

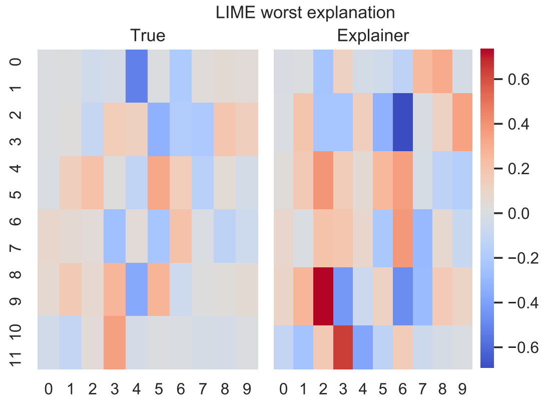


Figure C.69: The heatmap of explained effects of the worst explanation by `LIME` for a CNN trained on the MNIST dataset.

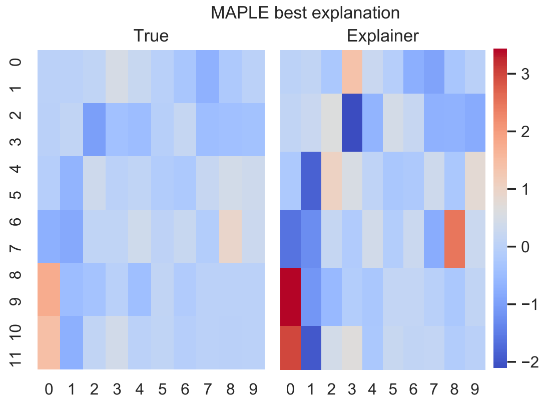


Figure C.70: The heatmap of explained effects of the best explanation by `MAPLE` for a CNN trained on the MNIST dataset.

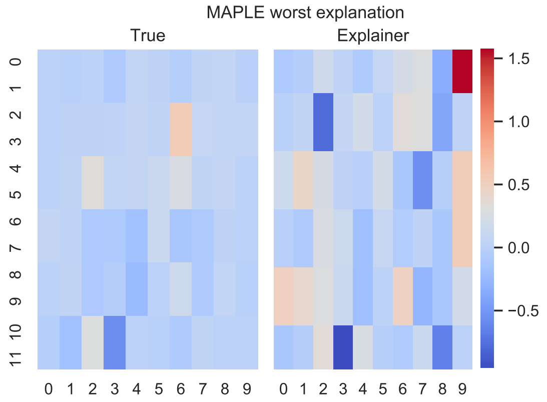


Figure C.71: The heatmap of explained effects of the worst explanation by `MAPLE` for a CNN trained on the MNIST dataset.

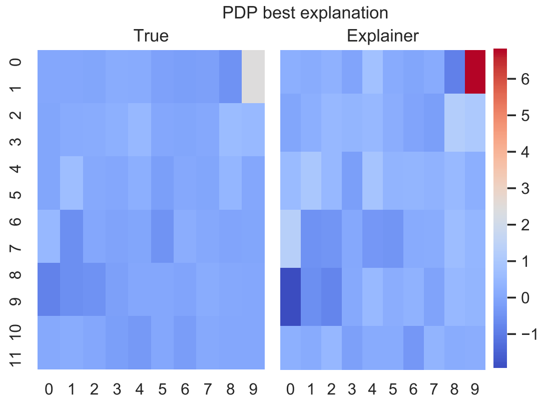


Figure C.72: The heatmap of explained effects of the best explanation by PDP for a CNN trained on the MNIST dataset.

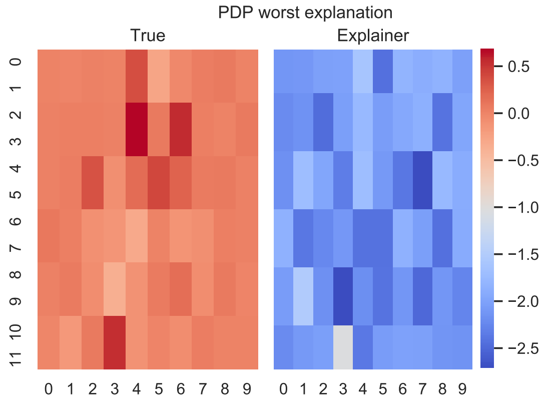


Figure C.73: The heatmap of explained effects of the worst explanation by PDP for a CNN trained on the MNIST dataset.

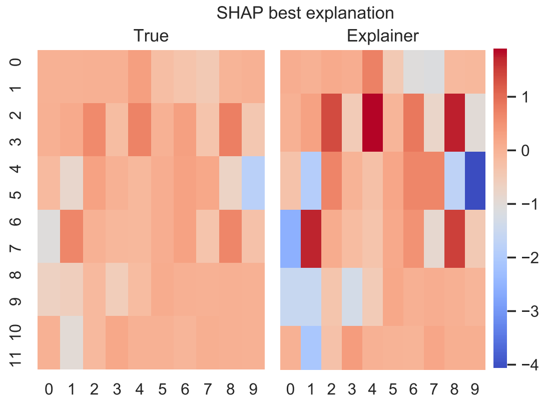


Figure C.74: The heatmap of explained effects of the best explanation by `SHAP` for a CNN trained on the MNIST dataset.

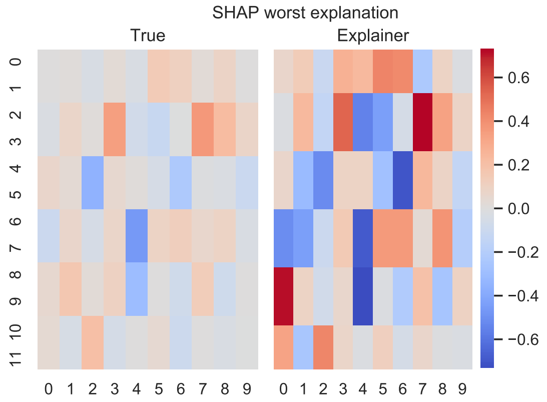


Figure C.75: The heatmap of explained effects of the worst explanation by `SHAP` for a CNN trained on the MNIST dataset.

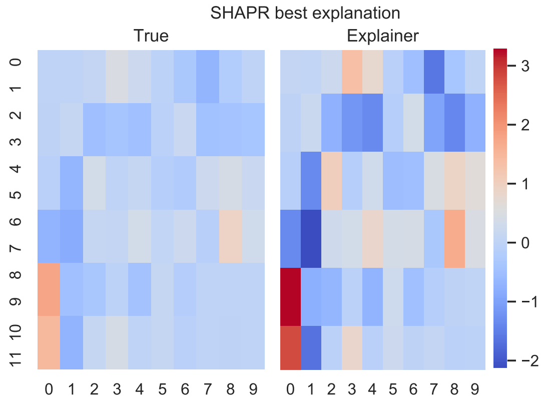


Figure C.76: The heatmap of explained effects of the best explanation by **SHAPR** for a CNN trained on the MNIST dataset.

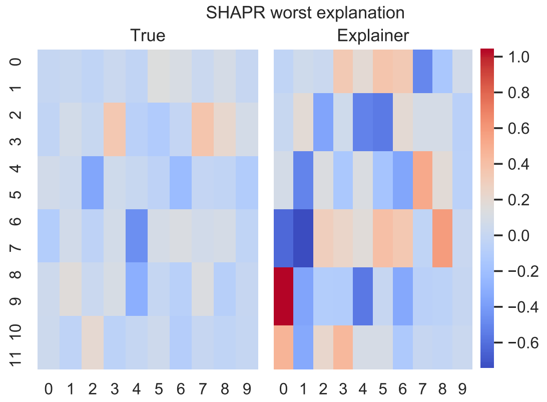


Figure C.77: The heatmap of explained effects of the worst explanation by **SHAPR** for a CNN trained on the MNIST dataset.

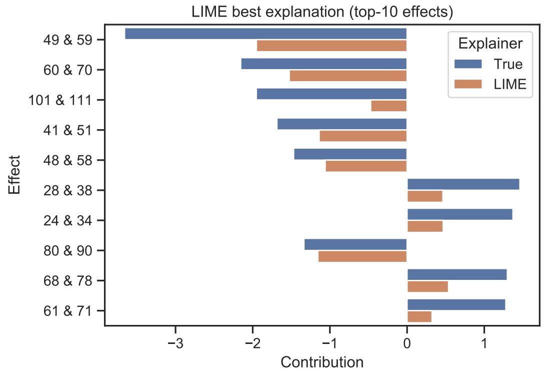


Figure C.78: The top-10 explained effects of the best explanation by `LIME` for a CNN trained on the MNIST dataset. Top effects are ranked by magnitude and the quality of explanation is ranked by mean cosine distance among all explained samples.

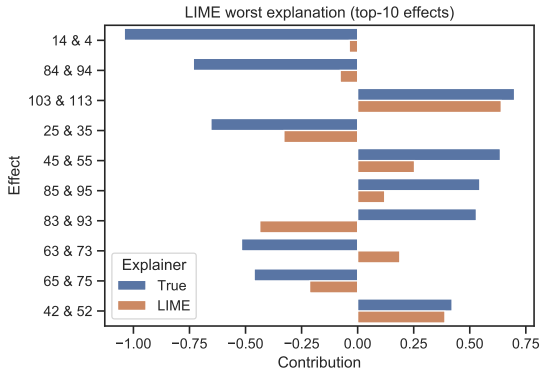


Figure C.79: The top-10 explained effects of the worst explanation by `LIME` for a CNN trained on the MNIST dataset. Top effects are ranked by magnitude and the quality of explanation is ranked by mean cosine distance among all explained samples.

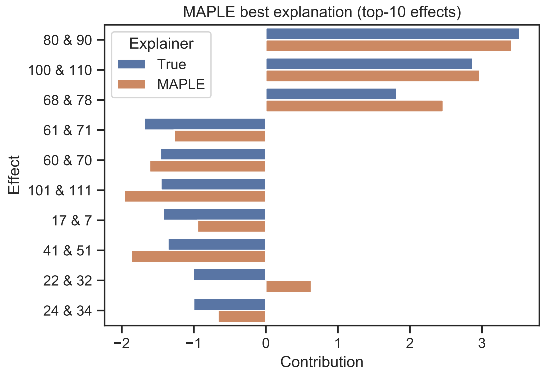


Figure C.80: The top-10 explained effects of the best explanation by `MAPLE` for a CNN trained on the MNIST dataset. Top effects are ranked by magnitude and the quality of explanation is ranked by mean cosine distance among all explained samples.

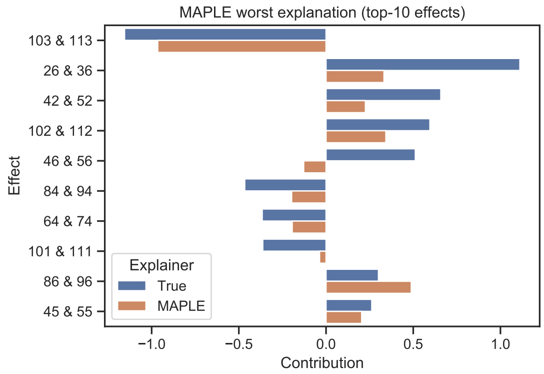


Figure C.81: The top-10 explained effects of the worst explanation by `MAPLE` for a CNN trained on the MNIST dataset. Top effects are ranked by magnitude and the quality of explanation is ranked by mean cosine distance among all explained samples.

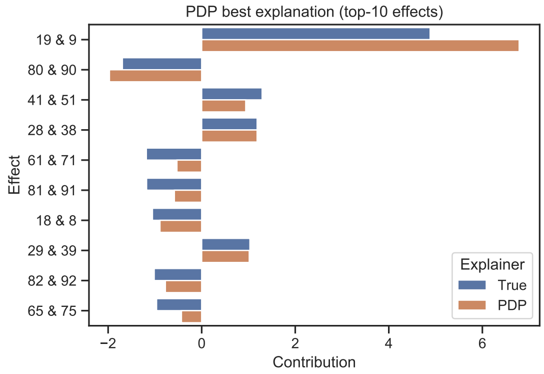


Figure C.82: The top-10 explained effects of the best explanation by `PDP` for a CNN trained on the MNIST dataset. Top effects are ranked by magnitude and the quality of explanation is ranked by mean cosine distance among all explained samples.

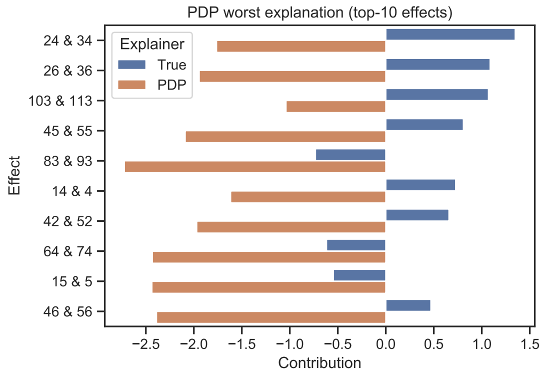


Figure C.83: The top-10 explained effects of the worst explanation by `PDP` for a CNN trained on the MNIST dataset. Top effects are ranked by magnitude and the quality of explanation is ranked by mean cosine distance among all explained samples.

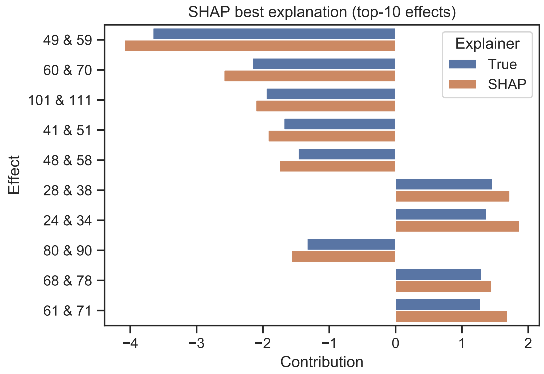


Figure C.84: The top-10 explained effects of the best explanation by SHAP for a CNN trained on the MNIST dataset. Top effects are ranked by magnitude and the quality of explanation is ranked by mean cosine distance among all explained samples.

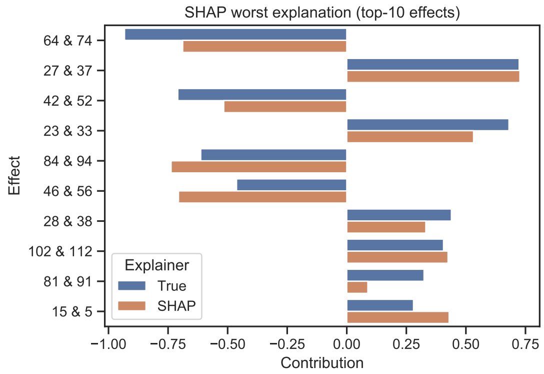


Figure C.85: The top-10 explained effects of the worst explanation by SHAP for a CNN trained on the MNIST dataset. Top effects are ranked by magnitude and the quality of explanation is ranked by mean cosine distance among all explained samples.

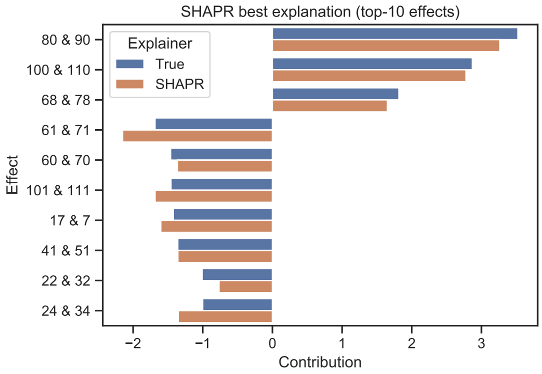


Figure C.86: The top-10 explained effects of the best explanation by **SHAPR** for a CNN trained on the MNIST dataset. Top effects are ranked by magnitude and the quality of explanation is ranked by mean cosine distance among all explained samples.

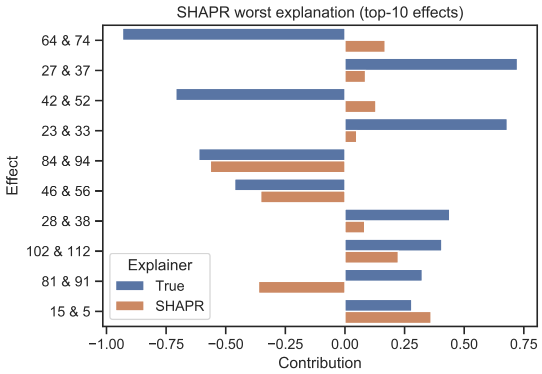


Figure C.87: The top-10 explained effects of the worst explanation by **SHAPR** for a CNN trained on the MNIST dataset. Top effects are ranked by magnitude and the quality of explanation is ranked by mean cosine distance among all explained samples.

## Appendix D Synthetic Model Generation

Synthetic models are generated as described by Algorithm 1, Generate-Model. This algorithm takes in three absolute parameters: the number of features, the number of dummy (unused) features, and the order of interactions. It also takes in two relative parameters: the percentage of nonlinear operators and the percentage of interaction terms. Generation is split into four phases: nonlinear main effects, linear main effects, nonlinear interaction effects, and linear interaction effects. These phases are marked by corresponding comments in the algorithm.

Before any phase, we select the unique features to use in the model, which is simply the $d$ features with the dummy features removed from consideration. After model generation, data is still drawn for these unused variables, but the model ignores it. For nonlinear main effects, we use at most the percentage of nonlinear operators times the number of features as the number of effects to generate. If this product is larger than the number of features, then we determine that the residual nonlinear operators will be applied to effects multiple times. For example, for $d = 2$ and a nonlinear percentage of 2 (200%), we may end up with something like $\cos(|x_1|) + \exp(\sqrt{x_2})$. This describes the steps where we place operators into some amount of bins (which is done as uniformly as possible with the values of each bin being an integer). Following this selection, we simply iterate over the unique features, applying the unary nonlinear operators to each, and add the result (still in symbolic form) to the expression. For linear main effects, we simply add the number of remaining features that have not had nonlinearities applied, if any, to the expression.

We have two parameters to consider for interaction effects: the interaction order (the number of features involved in each interaction) and the percentage of interaction terms (treated in the same manner as the percentage of nonlinear operators). We first select the unique interactions based on the number of interactions specified and the number of main effects. This is a simple way of constraining the sparsity of generated models — with too many interaction

terms, separation of effect contributions may not be possible by MatchEffects. The unique interactions selected are also naturally limited by the number of possible unique combinations given the number of features and the order of interactions. From these interactions, we select the number to be nonlinear in the exact same way as the main effects. However, we make choices from both unary and binary operators — binary operators are used to bridge together terms to form a whole effect and can include linear binary operators if the number of nonlinear operators is not sufficient to do so (*i.e.*, less than the number of features in an interaction minus one). Finally, we select the remaining linear interactions, choose linear interaction operators, and additionally add these to the expression.

See the previous supplemental content listing the unary and binary operators. The implementation of this algorithm has all randomness, *e.g.*, choices, seeded. For simplicity, the data structures (binary expression trees), random choices with operator weights, and valid domain checking are omitted from this algorithm.

**Algorithm 1:** GenerateModel: Generates a synthetic model satisfying various arguments

**Input:** $d$: the number of features

**Input:** $n_{dummy}$: the number of unused features

**Input:** $pct_{nonlinear}$: the percentage of nonlinearities used (relative to $d$)

**Input:** $pct_{interact}$: the percentage of interaction terms (relative to $d$)

**Input:** $order_{interact}$: the order of interaction terms ($\geq 2$)

**Result:** A randomly generated expression (model)

$features \leftarrow$ choose $(d - n_{dummy})$ unique features;

`// Initialize Expression`

$expr \leftarrow 0$;

`// Nonlinear Main Effects`

$n'_{main\_nonlinear} \leftarrow pct_{nonlinear} \times |features|$;

`// Number of terms`

$n_{main\_nonlinear} \leftarrow \min(n'_{main\_nonlinear}, |features|)$;

`// Each bin will on average contain` $n'_{main\_nonlinear}/n_{main\_nonlinear}$ `operators`

$ops_{main\_nonlinear} \leftarrow$ place $n'_{main\_nonlinear}$ unary nonlinear operators into $n_{main\_nonlinear}$ bins;

`// Cycle keeps track of the current element in a sequence, starting at the beginning if the previous element was at the end`

$main_{features} \leftarrow \text{cycle}(features)$;

**for** $i \in \{i \mid 1 \leq i \leq n_{main\_nonlinear}$ **do**

    `// Get the next feature in the cycle`

    $term \leftarrow$ next $main_{features}$;

    `// Apply nonlinearities`

    **for** $op \in ops_{main\_nonlinear}[i]$ **do**

        $term \leftarrow op(term)$;

    $expr \leftarrow expr + term$;

`// Linear Main Effects`

$n_{main\_linear} \leftarrow |features| - n_{main\_nonlinear}$;

**for** $i \in \{i \mid 1 \leq i \leq n_{main\_linear}\}$ **do**

    $feature \leftarrow$ next $main_{features}$;

    $expr \leftarrow expr + feature$;

`// Nonlinear Interaction Effects`



$n_{interact} \leftarrow \min\{pct_{interact} \times |features|, |features|\}$;

$n'_{interact\_nonlinear} \leftarrow pct_{nonlinear} \times n_{interact}$;

$interactions \leftarrow$ choose $n_{interact}$ unique feature pairs of size $order_{interact}$;

$n_{interact\_nonlinear} \leftarrow \min(n'_{interact\_nonlinear}, n_{interact})$;

`// Each is a unary/binary nonlinear operator or binary linear operator. #`

`// Linear Interaction Effects`

$n_{interact\_linear} \leftarrow n_{interact} - n_{interact\_nonlinear}$;

**for** $i \in \{i \mid 1 \leq i \leq n_{interact\_linear}\}$ **do**

  $interaction \leftarrow$ cycle(next $interact_{features}$);

  $ops_{interact\_linear} \leftarrow$ choose $|interaction| - 1$ linear non-additive binary operations;

  $term \leftarrow$ next $interaction$;

  **for** $op \in ops_{interact\_linear}$ **do**

    $feature \leftarrow$ next $interaction$;

    $term \leftarrow op(term, feature)$;

  $expr \leftarrow expr + feature$;

**return** $expr$
